# Supplementary material for: MMGR: Multi-Modal Generative Reasoning Benchmark and Evaluation
Source: arXiv:2512.14691 source file (2026-09-10)
Supplement: Supplementary file 1 [file X_appendix.tex]

\clearpage
\setcounter{page}{1}
\maketitlesupplementary

\section{Limitation}

Our benchmark still has several limitations. (i) We evaluate only at the API level for four proprietary models, so results may shift as providers update their systems and we cannot attribute errors to specific architectural choices. (ii) Automatic assessment relies mainly on a single VLM judge (Gemini-2.5-Pro) with limited manual spot-checking, leaving room for evaluator bias or hallucinated judgments. (iii) The current task suite emphasizes short, synthetic reasoning puzzles and controlled navigation scenes; it does not yet cover long-horizon, multi-agent, or highly realistic open-world footage. (iv) Evaluation is success-rate oriented and does not fully capture perceptual quality, temporal smoothness, or safety concerns, all of which matter for downstream deployment.

\section{Future Work}

To address these gaps, we plan to: (i) incorporate human evaluation and an ensemble of VLM judges to reduce single-judge bias; (ii) expand tasks toward longer temporal horizons, more diverse physics and social interactions, and higher-fidelity real-world videos; (iii) release reproducible data-generation and scoring pipelines so the community can re-run and extend the benchmark; (iv) explore automatic prompt tuning and self-correction loops to mitigate prompt sensitivity; and (v) build training/finetuning splits that encourage models to explicitly learn intermediate reasoning steps rather than relying on pattern matching.

\section{Statistics}

11111111 \\
11111111 \\
11111111 \\
11111111 \\
11111111 \\
11111111 \\
11111111 \\
11111111 \\
11111111 \\
11111111 \\
11111111 \\
11111111 \\
11111111 \\
11111111 \\
% 11111111 \\
% 11111111 \\
% 11111111 \\
% 11111111 \\
% 11111111 \\
% 11111111 \\
% 11111111 \\
% 11111111 \\
% 11111111 \\
% 11111111 \\

\section{Evaluation}
\label{sec:appendix_evaluation}

This section presents the complete evaluation results for all four models evaluated in our benchmark suite: Sora-2, Veo3-Preview, nano-banana, and gpt-4o-image. While the main paper (Table~\ref{tab:main_results}) focuses on Veo3-Preview and nano-banana, which represent the current state-of-the-art in video and image generation for reasoning tasks, we provide comprehensive results for all evaluated models here for completeness and future reference.

11111111 \\
11111111 \\
11111111 \\
11111111 \\
11111111 \\
11111111 \\
11111111 \\
11111111 \\
11111111 \\
11111111 \\
11111111 \\
11111111 \\
11111111 \\
11111111 \\
% 11111111 \\
% 11111111 \\
% 11111111 \\
% 11111111 \\
% 11111111 \\
% 11111111 \\
% 11111111 \\
% 11111111 \\
% 11111111 \\
% 11111111 \\

\begin{table}[!t] % 如果表格变窄了，可以考虑把 table* 改为 table 变为单栏，或者保持 table* 让其跨栏
\centering
\small
\caption{Overview of MMGR's \textit{three} task domains and the total number of samples per task. Together, these domains provide a comprehensive assessment across abstract reasoning, embodied navigation, and physical commonsense.}
\vspace{-1mm}
\label{tab:task_mapping}
\begin{tabular}{lc}
\toprule
\textbf{Benchmark Task Domain} & \textbf{\# Samples} \\
\midrule
\multicolumn{2}{l}{\textit{\textbf{Domain 1: Abstract Reasoning}}} \\
\quad Maze & $240$ \\
\quad Sudoku & $300$ \\
\quad ARC-AGI & $356$ \\
\quad Math & $327$ \\
\midrule
\multicolumn{2}{l}{\textit{\textbf{Domain 2: Embodied Navigation}}} \\
\quad 3D Real-World Navigation & $120$ \\
\quad Last-Mile Navigation (Ego-centric) & $120$ \\
\quad Top-down View Navigation & $120$ \\
\quad Simultaneous Localization and Generation & $120$ \\
\midrule
\multicolumn{2}{l}{\textit{\textbf{Domain 3: Physical Commonsense}}} \\
\quad Physical Concept & 50 \\
\quad Sports & 50 \\
\bottomrule
\end{tabular}
\vspace{-2mm}
\end{table}

\begin{table*}[ht!]
\centering
\caption{Complete zero-shot reasoning success rate (\%) for all evaluated models on our benchmark suite. Scores are calculated based on the Primary Metric defined for each task (detailed in Section~\ref{sec:tasks}). The highest score in each row is in \textbf{bold}.}
\label{tab:complete_results}
\small
\setlength{\tabcolsep}{6pt}
\begin{tabular}{ll cccc}
\toprule
& & \multicolumn{2}{c}{\textbf{Video Generation}} & \multicolumn{2}{c}{\textbf{Image Generation}} \\
\cmidrule(lr){3-4} \cmidrule(lr){5-6}
\textbf{Domain} & \textbf{Task} & Sora-2 & Veo3-Preview & nano-banana & gpt-4o-image \\
\midrule

% Abstract Reasoning Domain
\multirow{4}{*}{\shortstack{Abstract \\ Reasoning}} & Maze (Finish Task) & & 45.3 & & \\
& Sudoku (Valid Solution) & & & & \\
& ARC-AGI (Valid Solution) & & & & \\
& Math (Valid Solution) & & 7.78 & & \\
\midrule

% Embodied Navigation Domain (4 tasks now)
\multirow{4}{*}{\shortstack{Embodied \\ Navigation}} 
& Ego-centric Last-Mile Nav. (Reach Goal) & & & & \\
& Top-down Nav. (Reach Goal) & & & & \\
& 3D Real-World Nav. (Reach Goal) & & & & \\
& SLAG (Reach Goal \& Alignment) & & & & \\
\midrule

% Physical Commonsense Domain
\multirow{1}{*}{\shortstack{Physical Com.}} & Physical Commonsense & & & & \\
\midrule

\multicolumn{2}{l}{\textbf{Average Success Rate (\%)}} & & & & \\
\bottomrule
\end{tabular}
\end{table*}

\section{Physical Commonsense}
\label{sec:appendix_physics}

We introduce the Physical Commonsense domain to evaluate a model's foundational grasp of 'intuitive physics'~\citep{battaglia2013simulation, yi2019clevrer, wu2015galileo}-a core component of world modeling. This task serves as a direct probe for Physical Reasoning, challenging the model to generate videos that are not just photorealistic, but physically plausible~\citep{bear2021physion, riochet2021intphys, piloto2022intuitive}. It moves beyond static fidelity to test a model's understanding of concepts like gravity, momentum, collisions, and material properties (\eg, rigidity, fluids)~\citep{bakhtin2019phyre, allen2020rapid}. This domain also implicitly tests 3D Spatial Reasoning (how objects move and interact in 3D space) and Temporal Reasoning (the causal link between actions and reactions, \eg, A hits B, then B moves).

We structure our evaluation along two complementary axes: (1) \textit{Physical Concepts}-reusing the ontology from VideoPhy~\citep{videophy2024} to test fundamental physics principles across object interactions; and (2) \textit{Sports Scenarios}-evaluating compositional physical reasoning through synthesized sports contexts that naturally combine multiple physical laws.

\paragraph{Data Sources and Task Structure.}

\textbf{Physical Concepts Task.} We reuse the ontology from VideoPhy~\citep{videophy2024} to systematically test fundamental physics principles. VideoPhy provides a structured taxonomy covering three interaction types: \textit{Solid-Solid} interactions (143 captions, \eg, "A blender spins, mixing squeezed juice within it"), \textit{Solid-Fluid} interactions (146 captions, \eg, "A brave diver splashes into a pool from a great height"), and \textit{Fluid-Fluid} interactions (55 captions, \eg, "Honey diffusing into warm milk"). We also incorporate VideoPhy v2, which provides 600 unique test captions covering 197 unique physical actions across two main categories: Object Interactions and Sports/Physical Activities.

\textbf{Sports Scenarios Task.} To evaluate compositional physical reasoning, we synthesized additional sports-specific prompts that require integrating multiple physical laws. Our synthesized sports dataset includes: Ballet (12 captions: arabesque, pirouette, grand jeté, fouetté, etc.), Skiing (13 captions: downhill, jumping, turning, moguls, etc.), Diving (12 captions: straight dive, pike, somersault, platform dive, etc.), Swimming (13 captions: freestyle, butterfly, breaststroke, flip turn, etc.), and other sports contexts. Each sport naturally combines concepts like momentum, balance, fluid dynamics, and projectile motion.

\paragraph{Hard-Level Control.}

To generate a diverse and controllable set of evaluation cases, we structure our prompts along two primary axes, moving from basic physical properties to complex, compositional scenarios.

\begin{itemize} \item \textbf{Physical Concepts (Object Interaction Types):} Following the VideoPhy ontology~\citep{videophy2024}, we test three fundamental interaction types: \begin{itemize} \item \textit{Solid-Solid:} Interactions between rigid or semi-rigid objects (\eg, collisions, stacking, pushing). \item \textit{Solid-Fluid:} Interactions between solid objects and fluids (\eg, splashing, floating, pouring). \item \textit{Fluid-Fluid:} Interactions between different fluids or fluid states (\eg, mixing, diffusion, layering). \end{itemize} These interactions implicitly test core physics domains including statics (equilibrium, stability), dynamics (forces, momentum), kinematics (motion trajectories), object properties (rigidity, deformation), and hydrodynamics (fluid behavior, buoyancy). \item \textbf{Sports Scenarios (Compositional Contexts):} As a more challenging test, we evaluate sports scenarios that require the model to compose multiple physical laws simultaneously (\eg, gravity, collision, friction, and momentum) to achieve a goal. Our synthesized dataset spans diverse sports including aquatic sports (swimming, diving), precision sports (archery, ballet), winter sports (skiing), and other athletic activities. Each scenario tests the integration of multiple physical principles in realistic, goal-oriented contexts. \item \textbf{Interaction Complexity (3 levels):} For both axes, we vary complexity from Simple (\eg, single object motion), to Complex (\eg, multi-object interactions), to Chain-Reaction (\eg, cascading effects with temporal causality). \end{itemize}

\begin{table*}[h]
\begin{threeparttable}
\centering
\caption{Sample distribution for Physical Concepts task using VideoPhy ontology across interaction types and complexity levels. Total of 49 samples evaluated for veo3-preview model.}
\label{tab:physics_basic_distribution}
\begin{tabular}{lccc}
\toprule
\textbf{Interaction Type} & \textbf{Simple} & \textbf{Complex} & \textbf{Chain-Reaction} \\
\midrule
Solid-Solid & N/A & N/A & N/A \\
Solid-Fluid & N/A & N/A & N/A \\
Fluid-Fluid & N/A & N/A & N/A \\
\midrule
\textbf{Total} & \textbf{N/A} & \textbf{N/A} & \textbf{49*} \\
\bottomrule
\end{tabular}
\begin{tablenotes}
\small
\item \textbf{Note:} Physical Concepts scenarios follow the VideoPhy~\citep{videophy2024} ontology. Solid-Solid interactions test rigid body physics (collisions, momentum transfer, stacking). Solid-Fluid interactions evaluate object-fluid dynamics (splashing, floating, pouring). Fluid-Fluid interactions assess fluid mixing and layering behaviors. Complexity ranges from Simple (single interaction) to Chain-Reaction (cascading multi-object effects).
\item *Current evaluation includes 49 total samples across categories: Object Interactions (3), Sports (25), Sports \& Physical Activities (12), VideoPhysics (9). Detailed breakdown by interaction type and complexity level not available in current evaluation data. Only veo3-preview model has been evaluated; sora-2, nano-banana, and gpt-4o-image results are pending.
\end{tablenotes}
\end{threeparttable}
\end{table*}

\begin{table*}[h]
\begin{threeparttable}
\centering
\caption{Sample distribution for Sports Scenarios task across synthesized sports categories and complexity levels. Total of 37 sports-related samples evaluated for veo3-preview model.}
\label{tab:physics_sports_distribution}
\begin{tabular}{lccc}
\toprule
\textbf{Sport Category} & \textbf{Simple} & \textbf{Complex} & \textbf{Chain-Reaction} \\
\midrule
Ballet & N/A & N/A & N/A \\
Skiing & N/A & N/A & N/A \\
Diving & N/A & N/A & N/A \\
Swimming & N/A & N/A & N/A \\
Other Sports & N/A & N/A & N/A \\
\midrule
\textbf{Total} & \textbf{N/A} & \textbf{N/A} & \textbf{37*} \\
\bottomrule
\end{tabular}
\begin{tablenotes}
\small
\item \textbf{Note:} Sports Scenarios require compositional physical reasoning across multiple laws. Ballet tests balance, momentum, and rotational dynamics (arabesque, pirouette, grand jeté, fouetté). Skiing evaluates friction, gravity, and trajectory control (downhill, jumping, moguls). Diving assesses projectile motion, rotation, and fluid entry (pike, somersault, platform). Swimming tests fluid dynamics, propulsion, and body mechanics (freestyle, butterfly, breaststroke). Other sports include archery, gymnastics, and various athletic activities. Complexity ranges from Simple (basic movements) to Chain-Reaction (complex sequences with multiple physical transitions).
\item *Current evaluation includes 37 total sports-related samples: Sports (25), Sports \& Physical Activities (12). Detailed breakdown by specific sport type (Ballet, Skiing, Diving, Swimming) and complexity level not available in current evaluation data. Only veo3-preview model has been evaluated.
\end{tablenotes}
\end{threeparttable}
\end{table*}

\paragraph{Video Generation Prompt.} \label{sec:physics_video_prompt}

Representative textual prompts for each physical scenario type are reproduced in Section~\ref{sec:released_prompt_templates} (``Physical Commonsense'').

\paragraph{Image Generation Prompt.} \label{sec:physics_image_prompt}

\paragraph{Evaluation and Metrics.} \label{sec:physics_eval}

Given that "plausibility" is subjective and continuous, we use a VLM-based (Vision-Language Model) evaluator \citep{comanici2025gemini} prompted to act as a "physics expert." The VLM is given the generated video and a structured prompt with questions tailored to the specific scenario.

The evaluation prompt asks the VLM to answer a series of questions, such as:

"Does the video plausibly follow the laws of physics (\eg, gravity, momentum)?"

"In the collision, is momentum conserved (\eg, does the red ball move plausibly after being hit)?"

"Does the basketball's trajectory look like a real parabolic arc, or is it unnaturally linear or jerky?"

"Does any object 'glitch', 'teleport', or 'phase through' (pass through) another solid object?"

Based on the VLM's responses, we compute our primary and fine-grained metrics:

\begin{itemize} \item \textbf{Physical Plausibility (Primary Metric):} A 1-5 Likert scale score. This metric measures the overall physical correctness and realism of the generated interaction. A score of 5 indicates a perfectly plausible interaction that adheres to all expected physical laws. A score of 1 indicates a severe violation of physics (\eg, objects floating, passing through each other). \item \textbf{Collision/Phase Failure (Failure Mode):} A binary (0/1) metric that flags if the model failed basic object interaction, for example by allowing two solid objects to pass through one another. \item \textbf{Physics Violation (Failure Mode):} A binary (0/1) metric that flags a specific, non-collision-based violation (\eg, an object accelerating without a force, a ball bouncing higher than its drop height, incorrect gravity). \item \textbf{Prompt Adherence (Fine-grained Metric):} A binary (0/1) score that checks if the model generated the specific scenario (\eg, did it actually drop a feather and a ball, or just one?).
\end{itemize}

\begin{table*}[h!]
\begin{threeparttable}
\centering
\caption{Preliminary results for the Physical Commonsense task across different physical concepts.}
\label{tab:physics_results}
\begin{tabular}{@{}lcccc@{}}
\toprule
& \multicolumn{3}{c}{\textbf{Partial Score}} & \textbf{Primary Metric} \\
\cmidrule(lr){2-4}
\textbf{Model} & \textbf{Collision/Phase Failure} $\downarrow$ & \textbf{Physics Violation} $\downarrow$ & \textbf{Prompt Adherence} $\uparrow$ & \textbf{Physical Plausibility (1-5)} $\uparrow$ \\
\midrule
\multicolumn{5}{@{}l}{\textbf{Scenario Type: Basic Physics (Dynamics)}} \\
\multicolumn{5}{@{}l}{\quad \textbf{Video Models}} \\
\quad \quad veo3-preview & N/A & 28.57\% & 59.18\% & 3.57 \\
\quad \quad sora-2 & N/A & 14.00\% & 72.00\% & 4.30 \\

\multicolumn{5}{@{}l}{\textbf{Scenario Type: Compositional Sports}} \\
\multicolumn{5}{@{}l}{\quad \textbf{Video Models}} \\
\quad \quad veo3-preview & N/A & 28.57\% & 59.18\% & 3.57 \\
\quad \quad sora-2 & N/A & 14.00\% & 72.00\% & 4.30 \\
\bottomrule
\end{tabular}
\begin{tablenotes}
\small
\item \textbf{Note:} Results based on evaluation of 49 samples for veo3-preview model and 50 samples for sora-2 model. Metrics derived from evaluation data: Physics Violation = 100\% - Physics Accuracy (veo3-preview: 71.43\% accuracy → 28.57\% violation rate; sora-2: 86.00\% accuracy → 14.00\% violation rate). Prompt Adherence: veo3-preview = 59.18\% (29/49 samples), sora-2 = 72.00\% (36/50 samples). Physical Plausibility score converted from Physics Accuracy to 1-5 scale (veo3-preview: 71.43\% → 3.57/5; sora-2: 86.00\% → 4.30/5). Collision/Phase Failure metric not available in current evaluation format. nano-banana and gpt-4o-image models have not been evaluated for this task.
\end{tablenotes}
\end{threeparttable}
\end{table*}

\begin{figure*}[h]
    \centering
    \includegraphics[width=\textwidth, trim=0 0 0 0, clip]{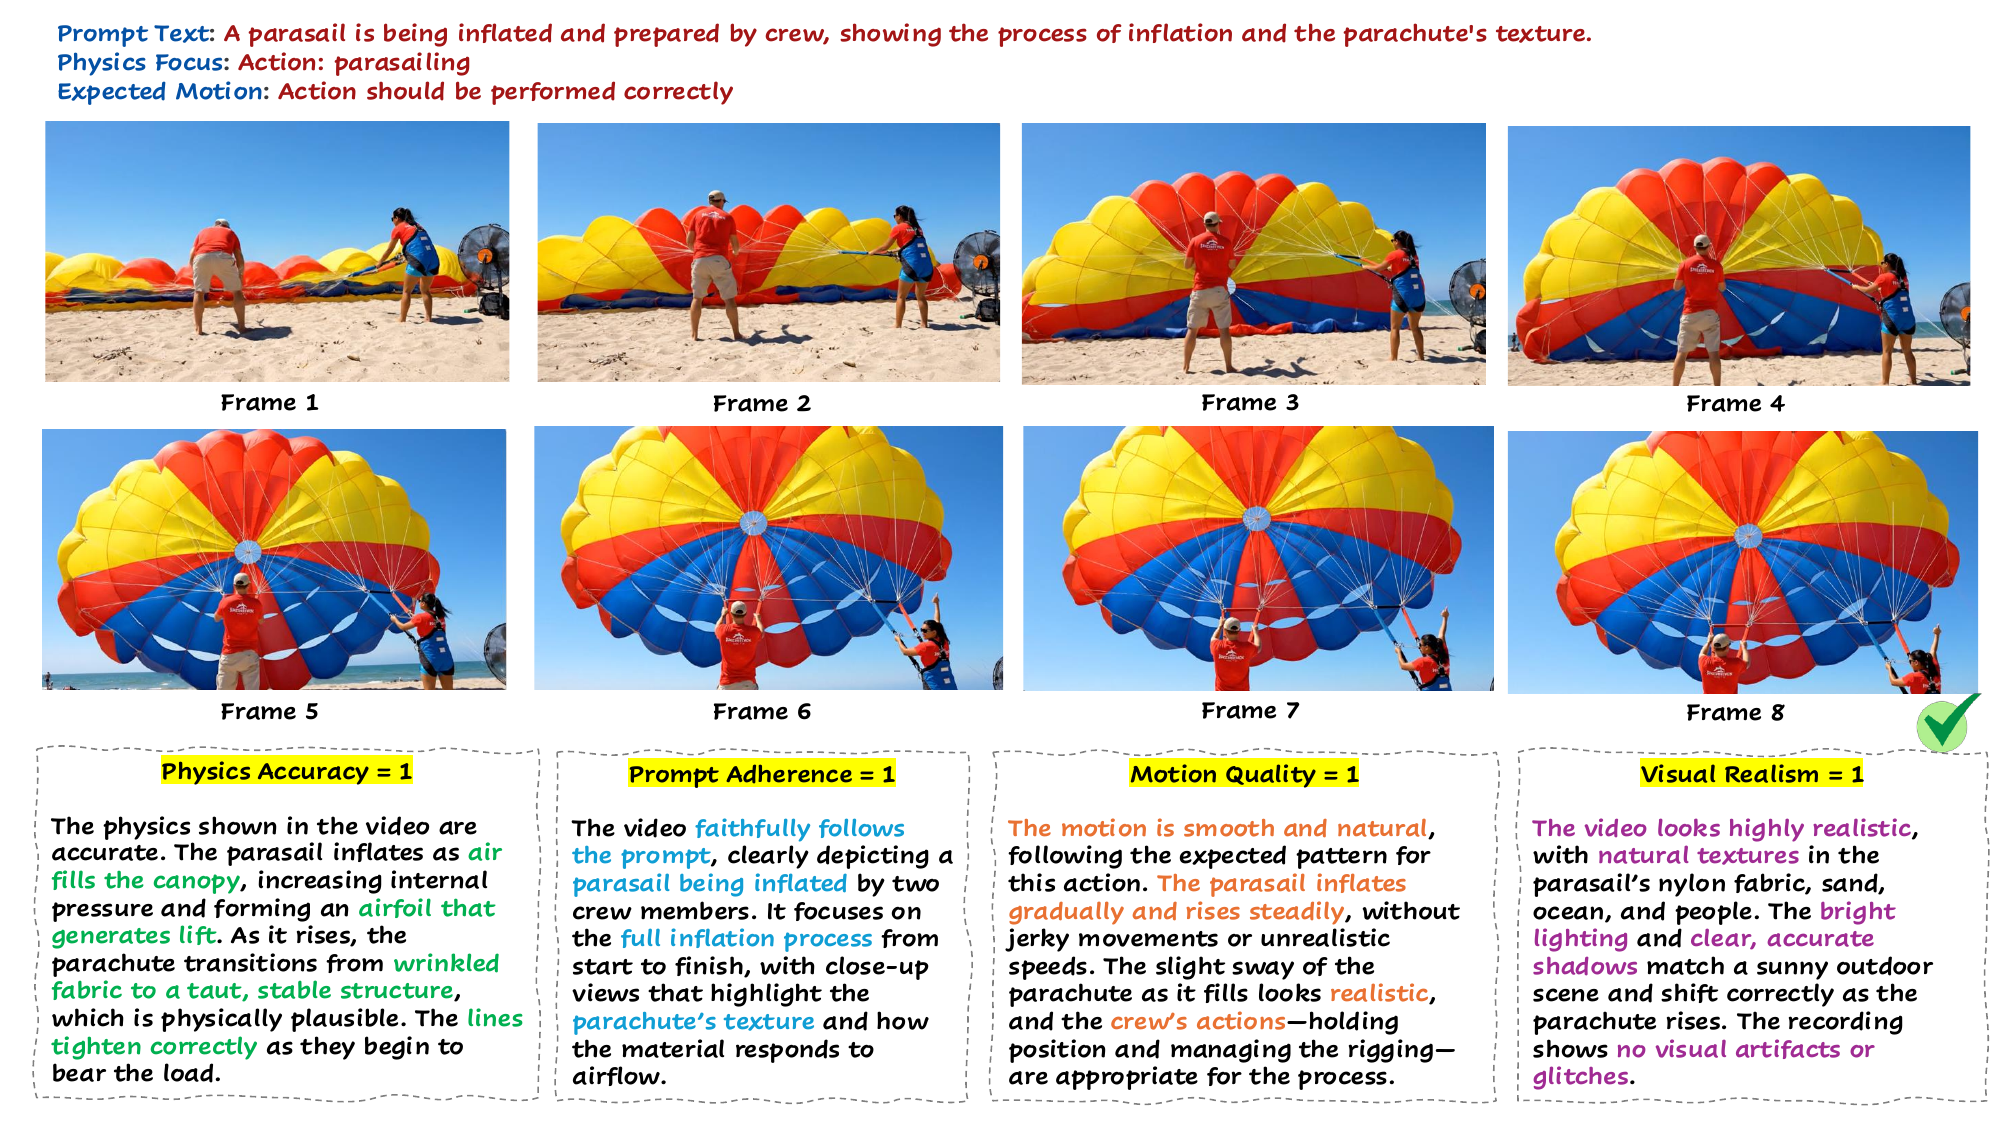}
    \vspace{-3mm}
    \caption{Case Study: Success case generated by \textit{Veo-3}.}
    % \vspace{-3mm}
    \label{fig:physics_case_study_1}
\end{figure*}

\begin{figure*}[h]
    \centering
    \includegraphics[width=\textwidth, trim=0 0 0 0, clip]{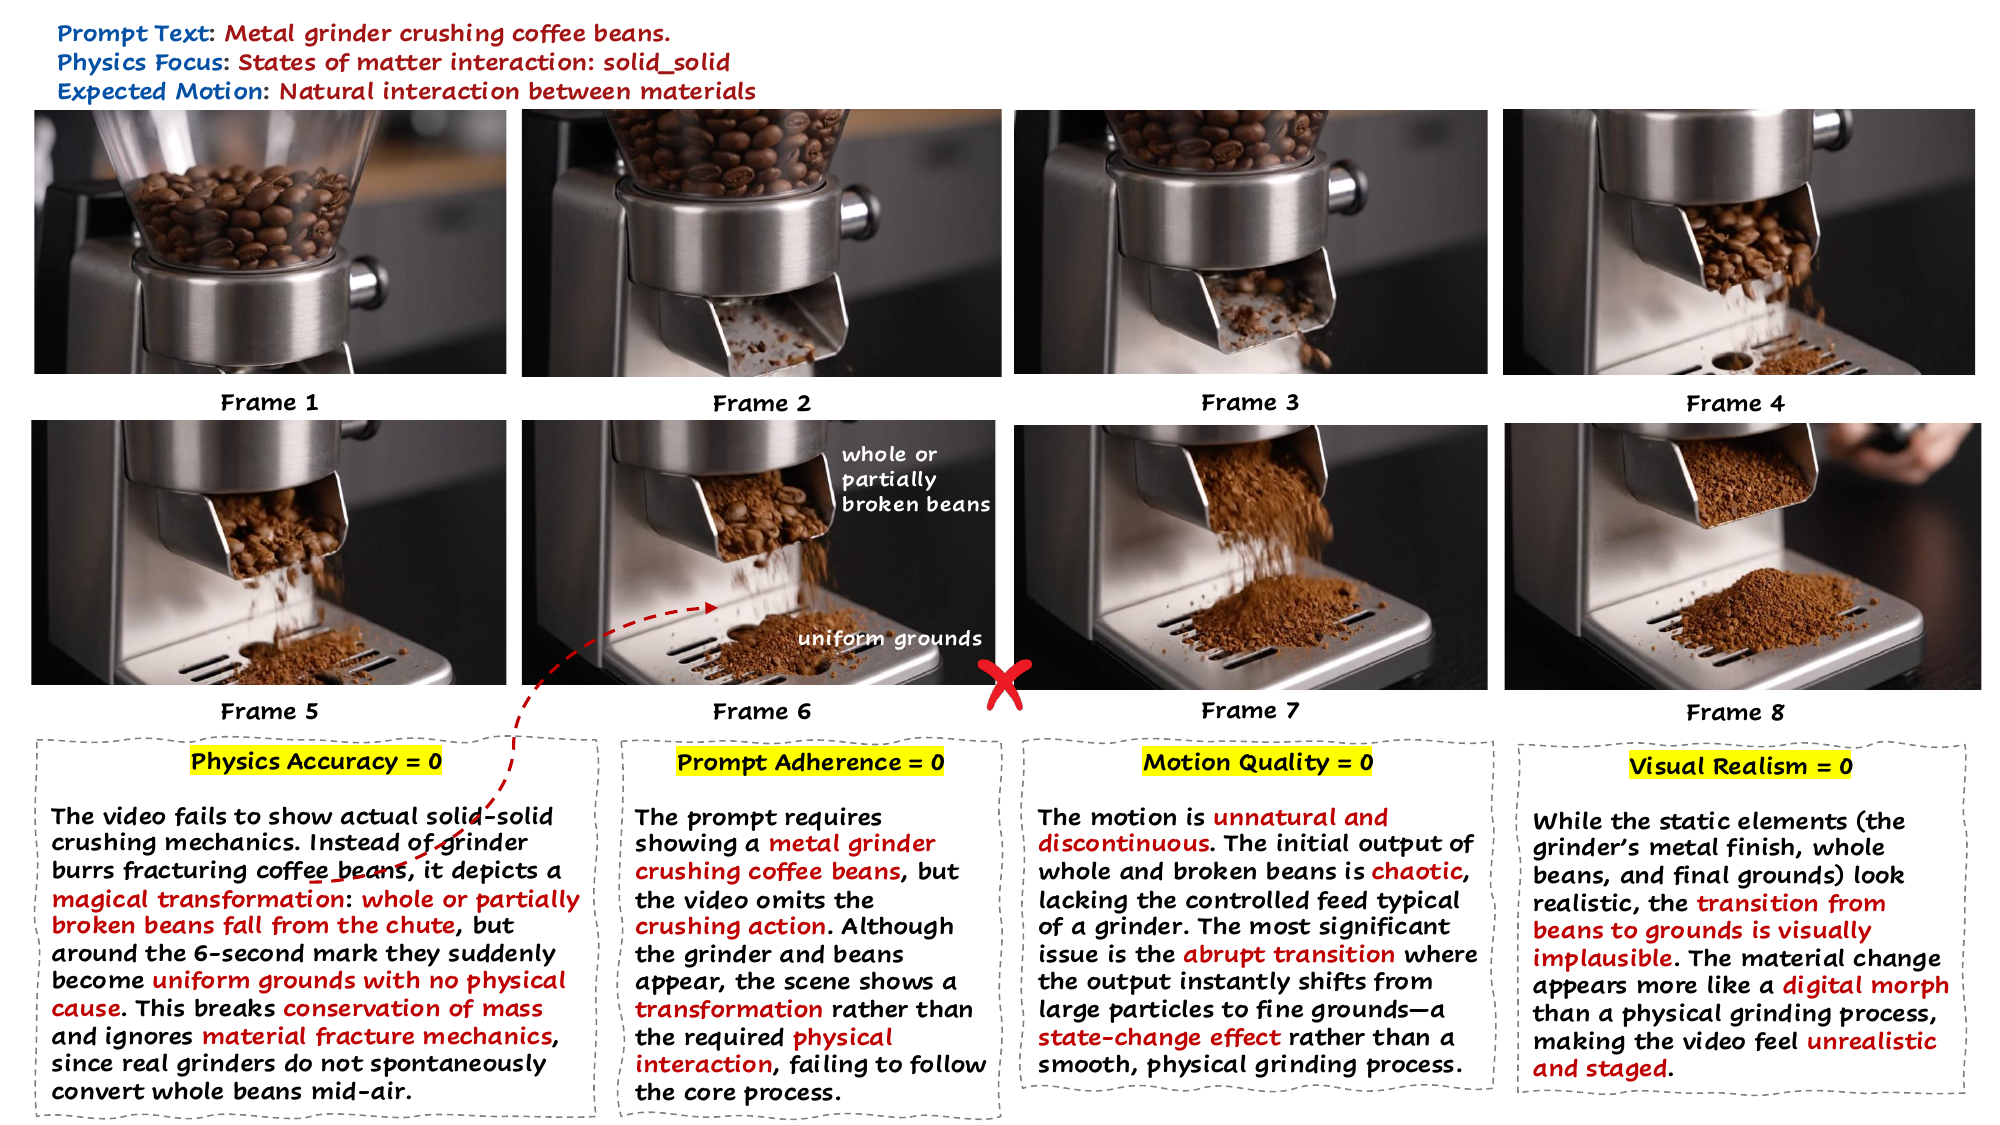}
    % \vspace{-2mm}
    \caption{Case Study: Failure case generated by \textit{Veo-3}.}
    \vspace{-3mm}
    \label{fig:physics_case_study_2}
\end{figure*}

\begin{figure*}[h]
    \centering
    \includegraphics[width=\textwidth, trim=0 0 0 0, clip]{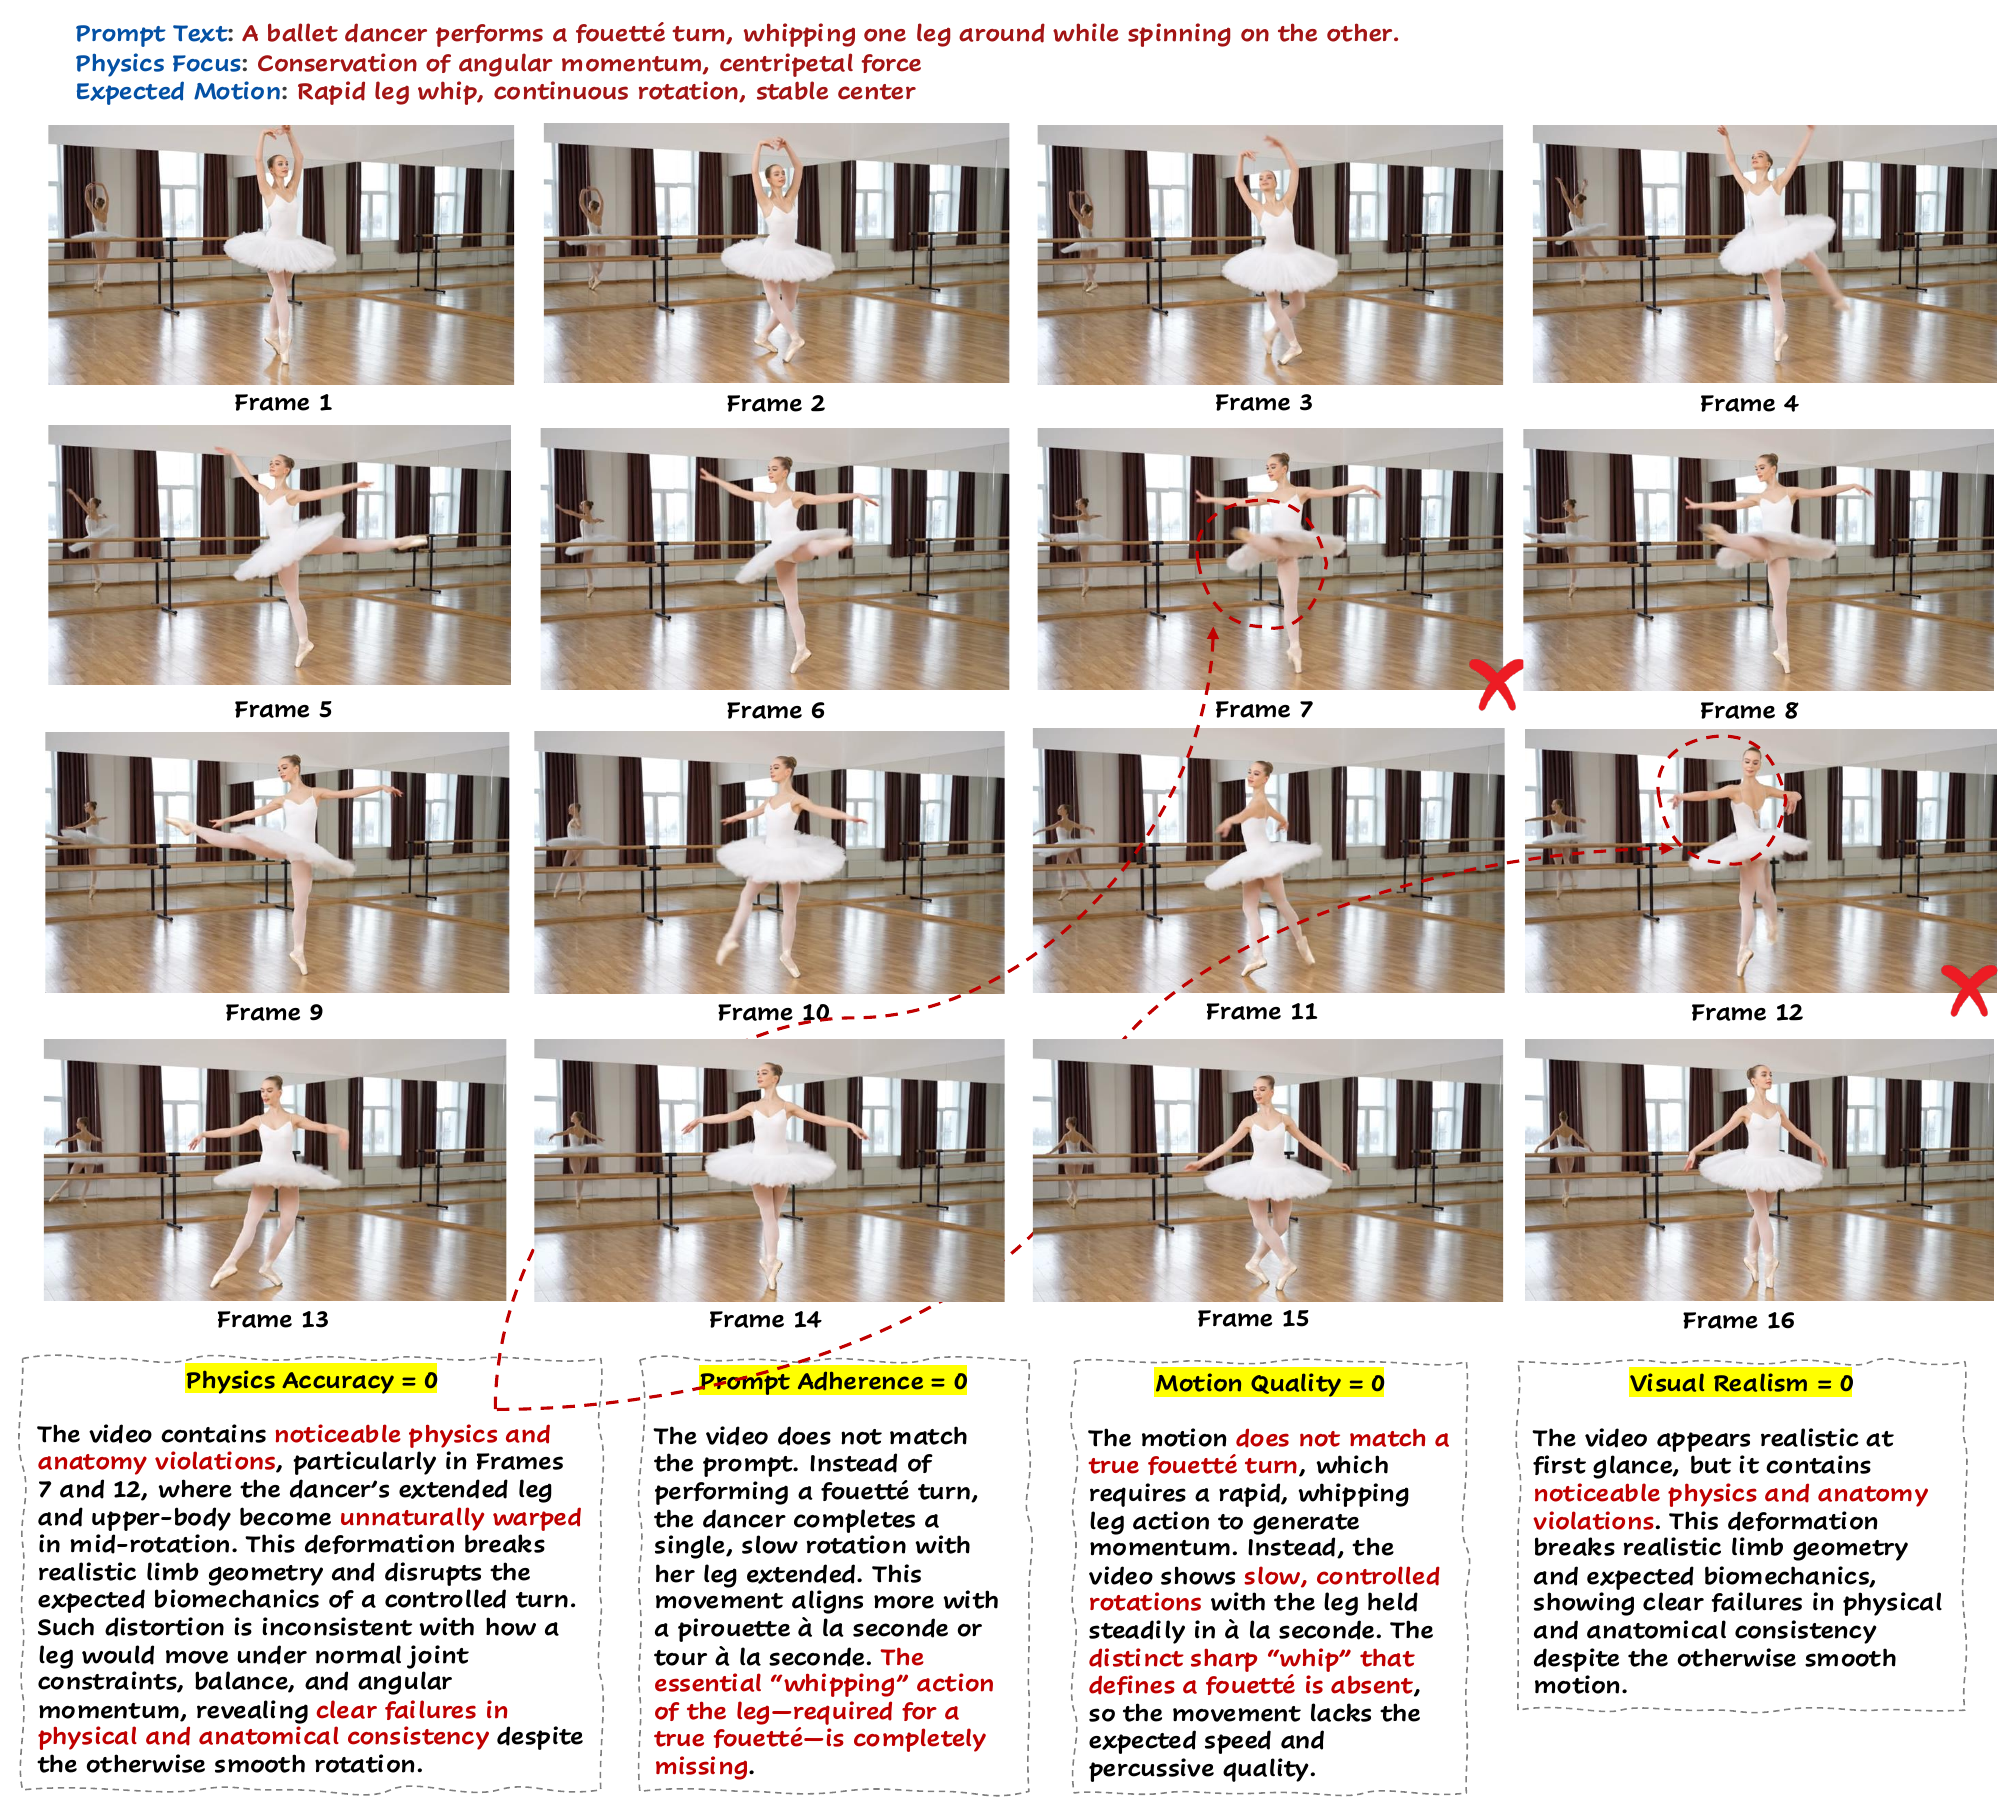}
    % \vspace{-2mm}
    \caption{Case Study: Failure case generated by \textit{Veo-3}.}
    \vspace{-3mm}
    \label{fig:physics_case_study_3}
\end{figure*}

\section{Human Annotation: Detailed Analysis} \label{sec:human_annotation_detailed}

We conducted systematic human evaluation with trained annotators to validate our benchmark. This section documents our annotation methodology, inter-annotator agreement, and comparison with automated evaluation.

\subsection{Annotation Interface and Protocol}

We developed a web-based interface with full video playback controls (frame-by-frame navigation, speed adjustment) and structured evaluation forms. Annotators assessed task completion, process correctness, visual quality, and failure modes with confidence ratings. Task-specific guidelines included evaluation criteria, visual examples, and edge case handling instructions.

\begin{figure*}[h]
  \centering
  \includegraphics[width=\textwidth]{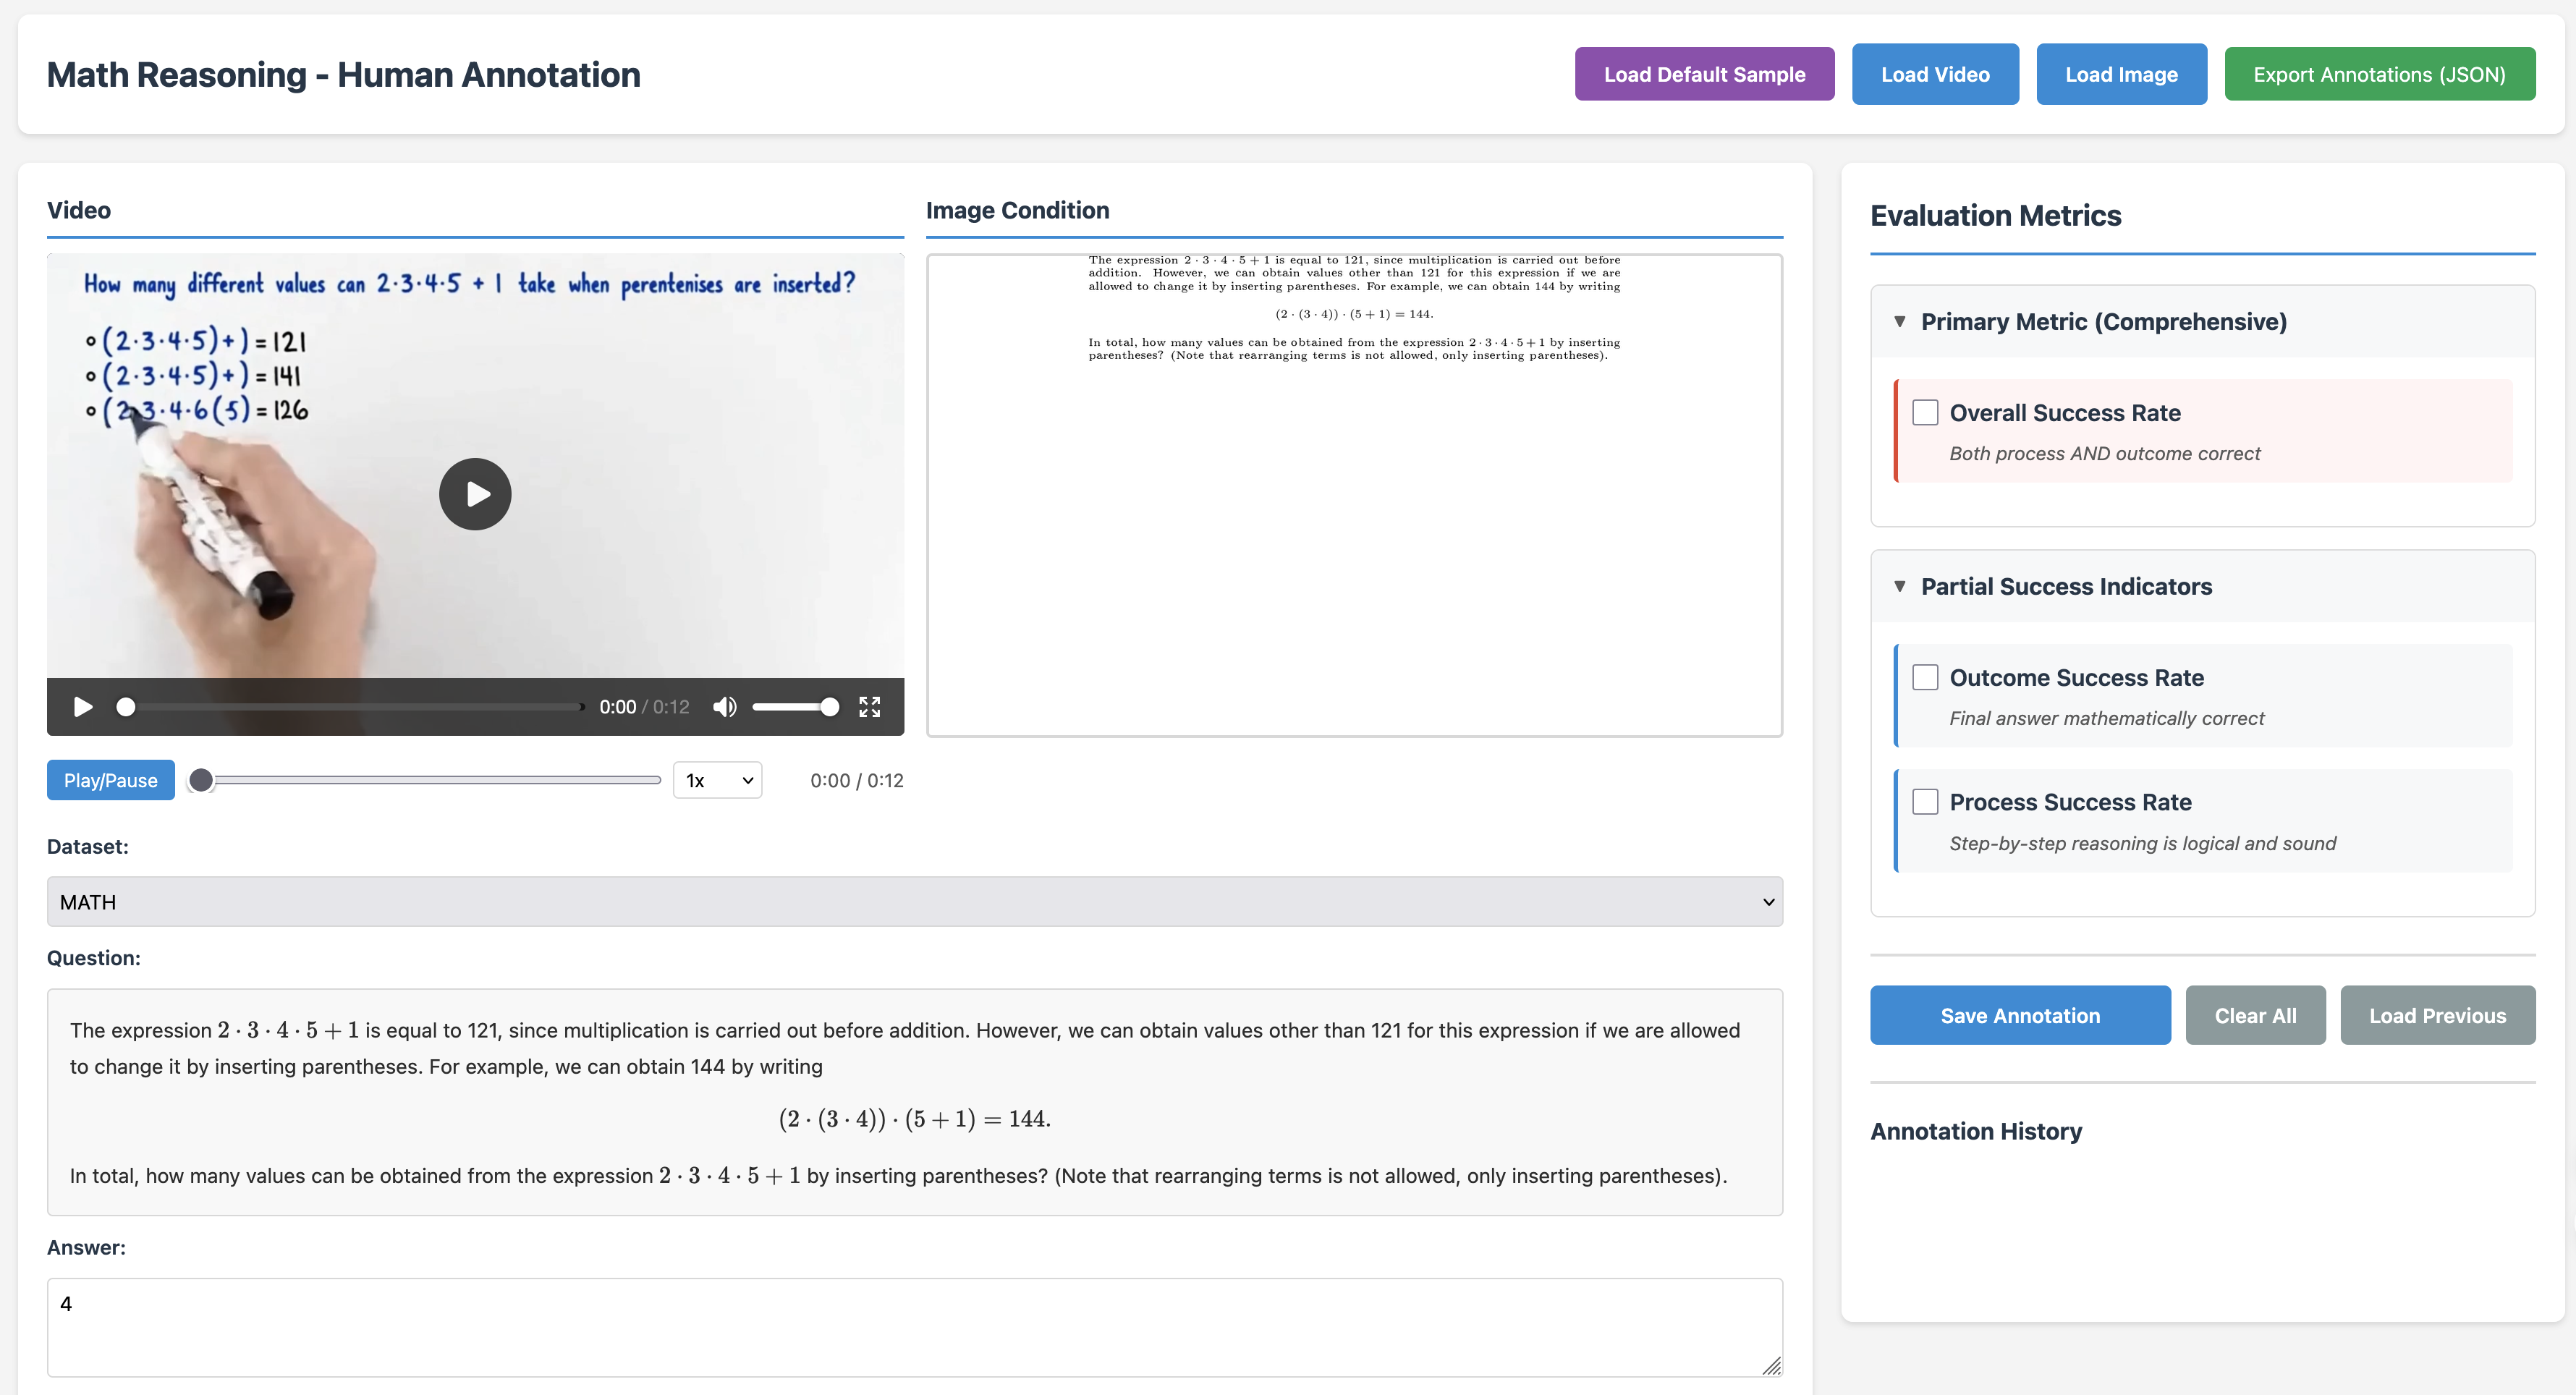}
  \caption{Example annotation interface for Math task showing the task prompt, generated video player, and structured evaluation form.}
  \label{fig:appendix_annotation_interface_math}
\end{figure*}

\begin{figure*}[h]
  \centering
  \includegraphics[width=\textwidth]{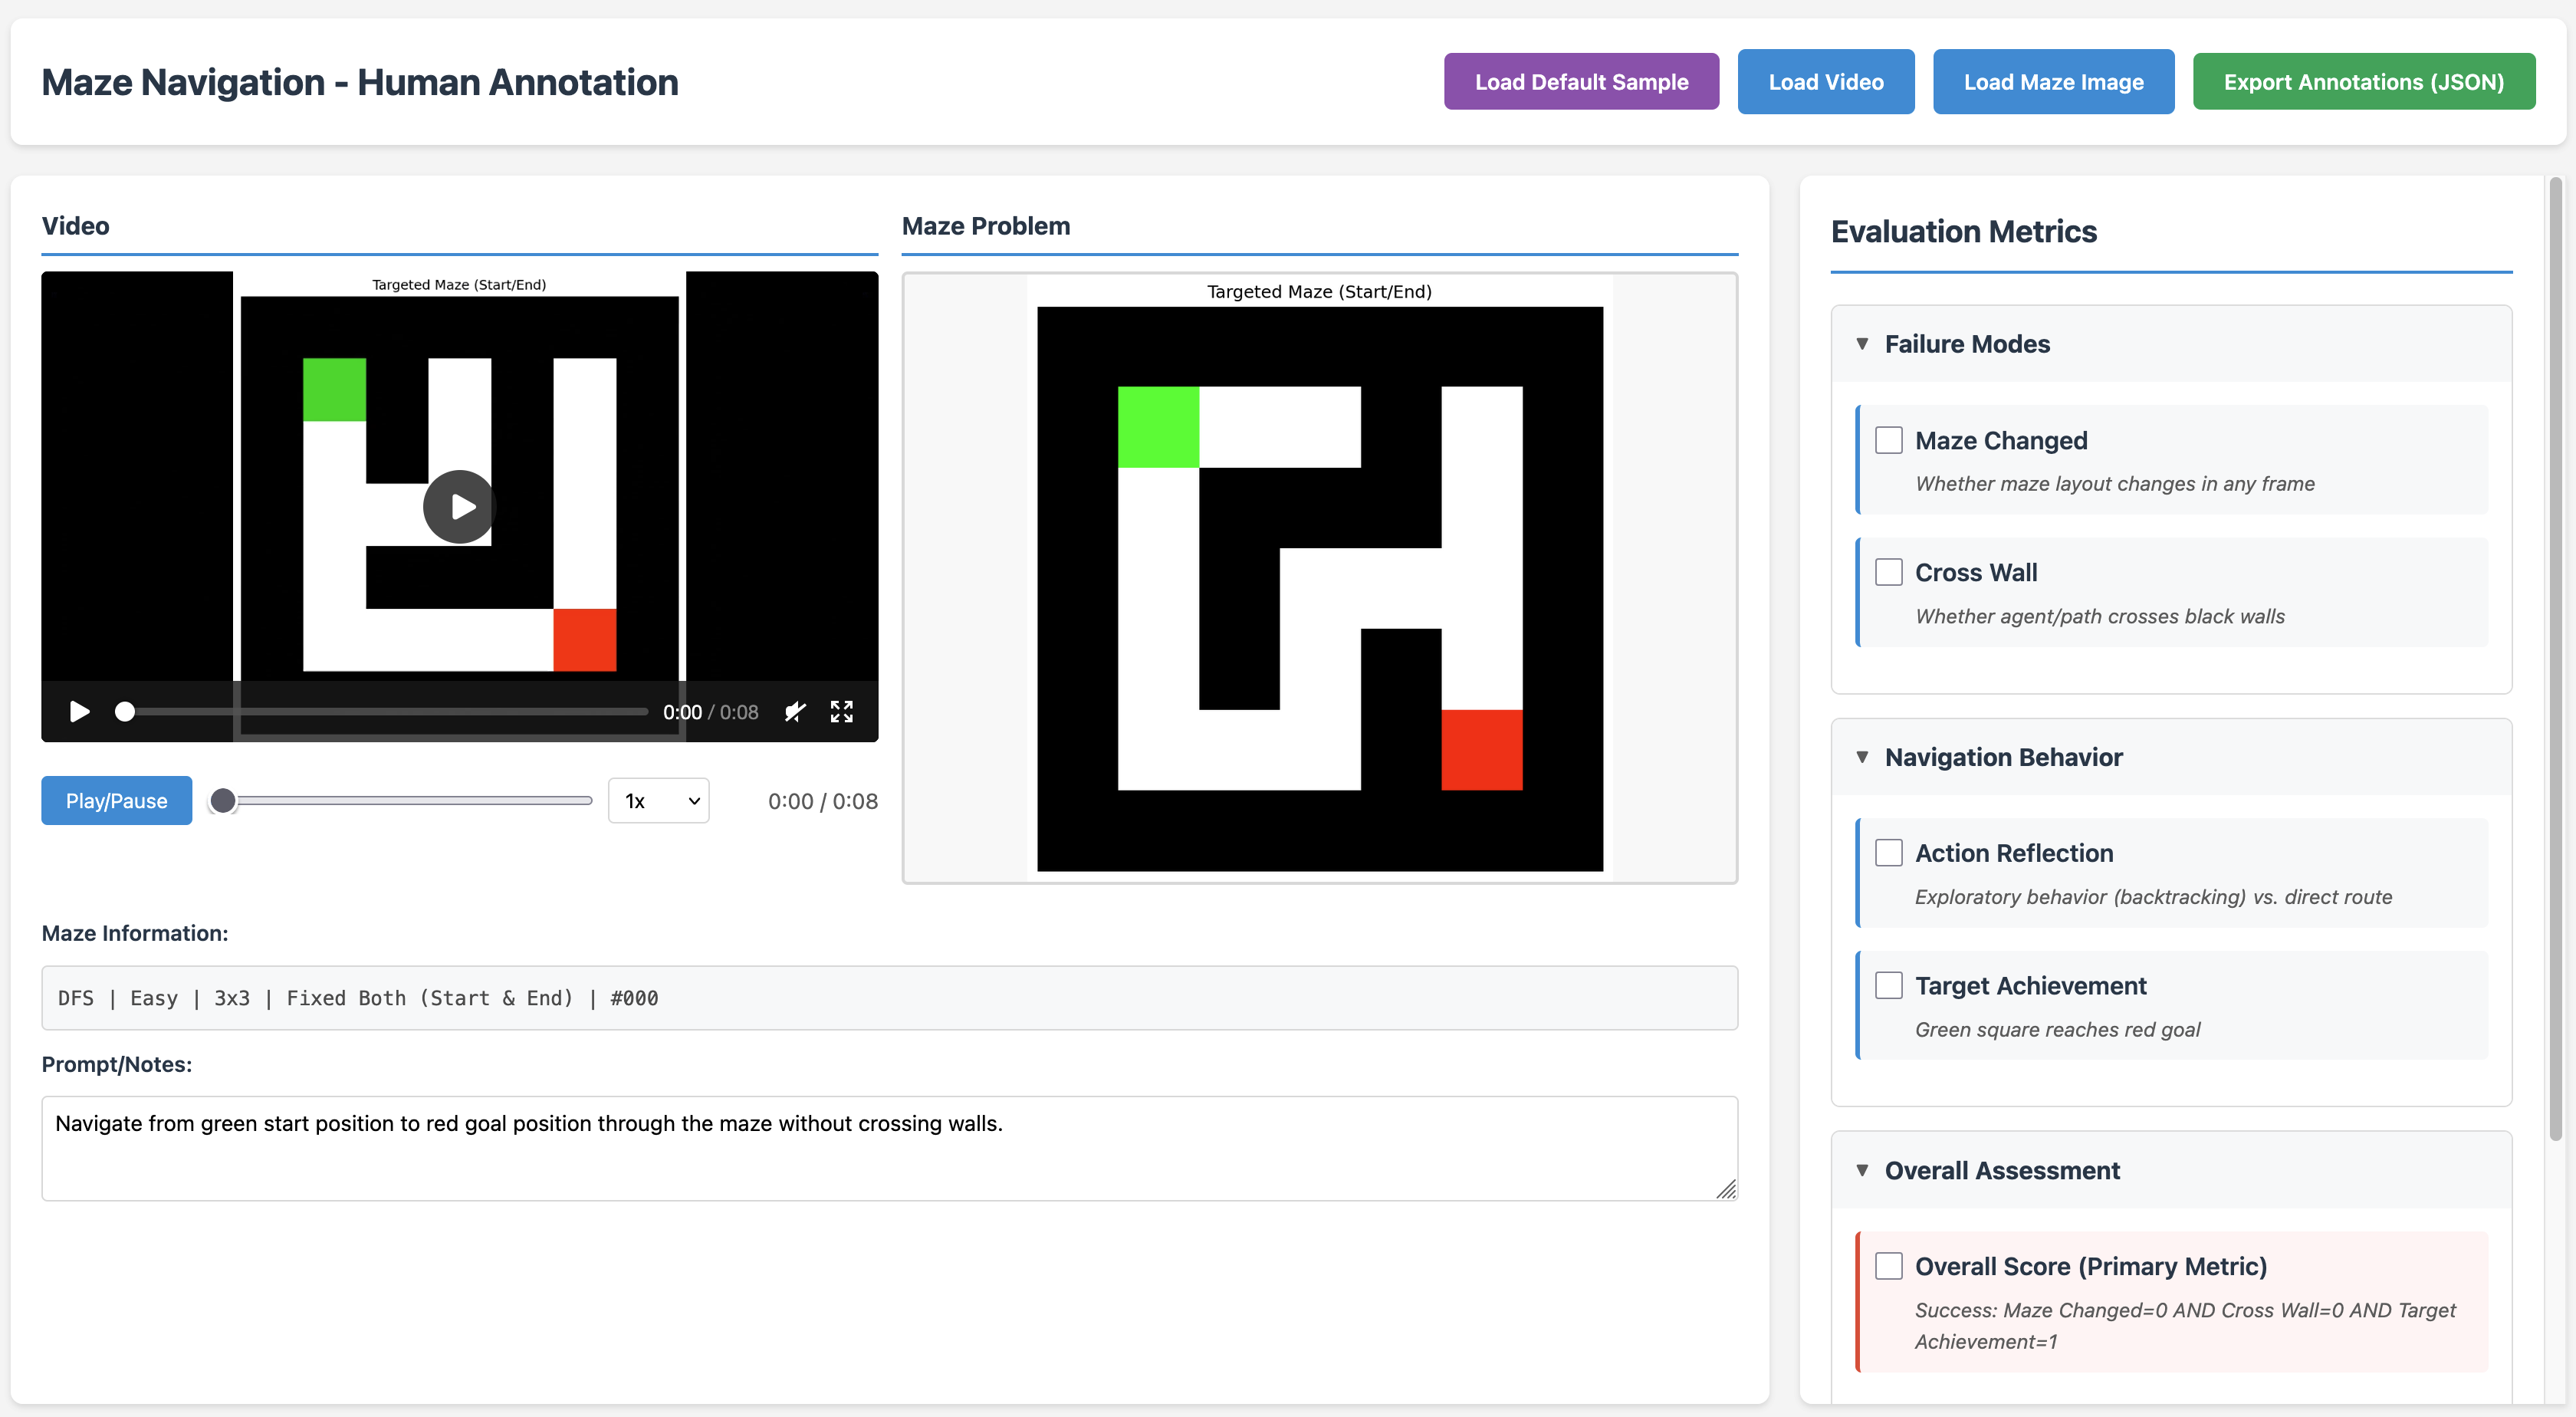}
  \caption{Example annotation interface for Maze task demonstrating frame-by-frame navigation controls for verifying path validity.}
  \label{fig:appendix_annotation_interface_maze}
\end{figure*}

\paragraph{Annotator Training and Quality Control.} We trained 6 annotators (computer science/cognitive science backgrounds) through a structured process: 4-hour training session, 50-video practice phase, calibration meeting, and 100-video pilot annotation. Only annotators achieving $\kappa > 0.70$ with gold standards proceeded to main annotation.

\paragraph{Annotation Process.} Each video (1,000+ total) received three independent annotations. Annotators worked in 2-hour sessions with mandatory breaks, blinded to model identity. We used majority voting for disagreement resolution (<3\% required senior arbitration) and median values for continuous scores.

\subsection{Task-Specific Guidelines}

\paragraph{Abstract Reasoning (Maze, Sudoku, Math).} Annotators verify intermediate steps and final solutions. For Maze: valid movements without wall-crossing; for Sudoku: rule compliance and grid completion; for Math: step-by-step correctness and final answer accuracy.

\paragraph{Embodied Navigation.} Annotators assess spatial consistency (smooth position changes), obstacle avoidance, goal reaching, and path sensibility across all navigation tasks.

\paragraph{Physical Commonsense.} Annotators evaluate gravity compliance, collision physics realism, object permanence, and absence of phase violations (objects passing through each other).

\subsection{Inter-Annotator Agreement}

Table~\ref{tab:appendix_iaa_detailed} shows Cohen's kappa ($\kappa$) for pairwise agreement across all tasks.

\begin{table}[h]
\centering
\caption{Detailed inter-annotator agreement (Cohen's kappa) for each task. Mean $\kappa$ and range across all annotator pairs are reported.}
\label{tab:appendix_iaa_detailed}
\begin{tabular}{@{}lcc@{}}
\toprule
\textbf{Task} & \textbf{Mean $\kappa$} & \textbf{Range} \\
\midrule
Maze & 0.82 & 0.78 - 0.86 \\
Sudoku & 0.85 & 0.82 - 0.88 \\
ARC-AGI & 0.76 & 0.72 - 0.80 \\
Math & 0.79 & 0.75 - 0.83 \\
Top-down Navigation & 0.77 & 0.73 - 0.81 \\
3D Real-World Navigation & 0.75 & 0.71 - 0.79 \\
SLAG & 0.73 & 0.69 - 0.77 \\
Last-Mile Navigation & 0.74 & 0.70 - 0.78 \\
Physical Commonsense & 0.71 & 0.67 - 0.75 \\
\midrule
\textbf{Overall Mean} & \textbf{0.78} & \textbf{0.71 - 0.85} \\
\bottomrule
\end{tabular}
\end{table}

\paragraph{Key Findings.} Objective tasks (Sudoku: $\kappa = 0.85$, Maze: $\kappa = 0.82$) achieved highest agreement due to clear success criteria. Reasoning tasks (Math: $\kappa = 0.79$, ARC-AGI: $\kappa = 0.76$) showed moderate agreement, with disagreements on partial solutions. Navigation tasks ($\kappa = 0.73$-$0.77$) had edge case ambiguities. Physical Commonsense ($\kappa = 0.71$) had lowest agreement due to subjective plausibility judgments. All tasks achieved substantial agreement ($\kappa > 0.70$), validating annotation quality.

\subsection{AutoEval vs HumanEval}

We compared AutoEval (Gemini 2.5-Pro) with HumanEval on 200+ videos per task. Table~\ref{tab:appendix_autoeval_correlation} shows correlation metrics.

\begin{table}[h]
\centering
\caption{Correlation between AutoEval and HumanEval scores across tasks.}
\label{tab:appendix_autoeval_correlation}
\resizebox{\columnwidth}{!}{
\begin{tabular}{@{}lccc@{}}
\toprule
\textbf{Task} & \textbf{Pearson $r$} & \textbf{MAE (0-100 scale)} & \textbf{AutoEval Bias} \\
\midrule
Maze & 0.73 & 12.5 & +8.2 (overestimate) \\
Sudoku & 0.89 & 6.3 & +2.1 (slight overestimate) \\
ARC-AGI & 0.68 & 15.7 & +10.5 (overestimate) \\
Math & 0.71 & 13.9 & +9.8 (overestimate) \\
Top-down Navigation & 0.76 & 11.2 & +5.4 (moderate overestimate) \\
3D Real-World Navigation & 0.69 & 16.3 & +12.7 (overestimate) \\
SLAG & 0.65 & 18.1 & +14.2 (strong overestimate) \\
Last-Mile Navigation & 0.72 & 14.6 & +11.3 (overestimate) \\
Physical Commonsense & 0.78 & 10.8 & +6.9 (moderate overestimate) \\
\midrule
\textbf{Overall} & \textbf{0.73} & \textbf{13.3} & \textbf{+9.0} \\
\bottomrule
\end{tabular}
}
\end{table}

\paragraph{Key Findings.} AutoEval shows strong alignment on objective tasks (Sudoku: $r = 0.89$, MAE = 6.3), moderate alignment on reasoning tasks (Maze, Math: $r = 0.71$-$0.73$), and weaker alignment on spatial/abstract tasks (SLAG, ARC-AGI, 3D Nav: $r = 0.65$-$0.69$, MAE = 15.7-18.1).

AutoEval systematically overestimates performance (average +9.0 points), most severely on SLAG (+14.2), 3D Navigation (+12.7), and ARC-AGI (+10.5). This stems from difficulty detecting subtle spatial inconsistencies, goal-reaching ambiguities, and abstract pattern violations.

\paragraph{Discrepancy Sources.} Three primary factors drive discrepancies: (1) \textbf{Frame sampling}: AutoEval samples 8-16 frames, missing transient violations that humans catch with continuous playback; (2) \textbf{Spatial reasoning}: humans excel at detecting subtle position jumps and size changes; (3) \textbf{Partial credit}: humans apply stricter standards for partial solutions.

\paragraph{Evaluation Strategy.} AutoEval excels at scalability, consistency, and objective tasks. HumanEval excels at temporal reasoning, spatial precision, and nuanced judgment. We recommend: AutoEval for large-scale screening and objective tasks; HumanEval for final benchmarks and complex reasoning; combined approaches for comprehensive coverage.

\paragraph{ARC-AGI Detailed Analysis.} We compared Gemini AutoEval with human annotations on 98 ARC-AGI cases across four metrics: pattern recognition, grid integrity, color accuracy, and valid solution.

\begin{table}[h]
\centering
\caption{Inter-evaluator agreement between Gemini and Human annotations.}
\label{tab:gemini_human_agreement}
\small
\begin{tabular}{@{}lccc@{}}
\toprule
\textbf{Metric} & \textbf{Kappa ($\kappa$)} & \textbf{Agreement Rate} & \textbf{Interpretation} \\
\midrule
Pattern Recognition & 0.273 & 78.6\% & Fair (best alignment) \\
Grid Integrity & 0.220 & 67.3\% & Fair \\
Color Accuracy & 0.093 & 74.5\% & Slight \\
Valid Solution & 0.000 & 94.9\% & Poor (no variance in human) \\
\bottomrule
\end{tabular}
\end{table}

Pattern recognition shows best agreement ($\kappa = 0.273$). High raw agreement (67-95\%) reflects mutual agreement on failures. Humans marked zero valid solutions while Gemini marked 5.1\%, indicating human strictness. Color accuracy shows poor agreement ($\kappa = 0.093$).

\begin{table}[h]
\centering
\caption{Pearson correlation between Gemini and Human evaluations.}
\label{tab:gemini_human_correlation}
\small
\begin{tabular}{@{}lcc@{}}
\toprule
\textbf{Metric} & \textbf{Pearson $r$} & \textbf{$p$-value} \\
\midrule
Pattern Recognition & 0.277 & 0.006** \\
Grid Integrity & 0.222 & 0.028* \\
Color Accuracy & 0.118 & 0.245 (n.s.) \\
Valid Solution & --- & --- (no variance) \\
\bottomrule
\multicolumn{3}{@{}l@{}}{\small *$p < 0.05$, **$p < 0.01$, n.s. = not significant}
\end{tabular}
\end{table}

Pattern recognition ($r = 0.277$, $p = 0.006$) and grid integrity ($r = 0.222$, $p = 0.028$) show significant correlations. Color accuracy lacks correlation ($r = 0.118$, $p = 0.245$), confirming divergent standards.

\begin{table}[h]
\centering
\caption{Pass rates (percentage marked as correct) by evaluator.}
\label{tab:gemini_human_performance}
\small
\begin{tabular}{@{}lccc@{}}
\toprule
\textbf{Metric} & \textbf{Human} & \textbf{Gemini} & \textbf{Difference} \\
\midrule
Valid Solution & 0.0\% & 5.1\% & +5.1\% \\
Pattern Recognition & 20.4\% & 15.3\% & -5.1\% \\
Grid Integrity & 26.5\% & 32.7\% & +6.1\% \\
Color Accuracy & 24.5\% & 7.1\% & \textbf{-17.3\%}** \\
\bottomrule
\multicolumn{4}{@{}l@{}}{\small **Statistically significant (McNemar test, $p = 0.0014$)}
\end{tabular}
\end{table}

Color accuracy shows a significant 17.3\% gap (Human: 24.5\%, Gemini: 7.1\%; $p = 0.0014$), with humans accepting "close enough" matches while Gemini enforces strict pixel-perfect matching. Pattern recognition shows best agreement (71\% mutual incorrect, 7\% mutual correct).

\textbf{Key Implications:} Gemini is reliable for structural metrics (pattern recognition, grid integrity) but overly strict on perceptual attributes (color). Calibration or hybrid evaluation (Gemini for structure, humans for perception) recommended when color assessment is critical.

\subsection{Common Failure Modes}

Human annotation identified three primary failure categories:

\paragraph{Abstract Reasoning.} Visually plausible but logically incorrect (42\% Maze, 38\% Sudoku); abandonment after partial progress (23\% Math, 19\% ARC-AGI); rule violation blindness (31\% Sudoku, 28\% Maze).

\paragraph{Spatial Reasoning.} Position inconsistency/teleportation (35\%); collision violations/wall-passing (27\%); goal confusion (18\%).

\paragraph{Physical Reasoning.} Gravity violations (22\%); collision phase-through (33\%); momentum violations (28\%).

These patterns reveal limitations in video models' world models and reasoning capabilities.

\begin{table*}[t!]
\centering
\caption{Index of all task prompts in the appendix. Each task includes video generation, image generation, and evaluation prompts detailed in their respective sections.}
\label{tab:prompt_index}
\small
\begin{tabular}{llllll}
\toprule
\textbf{Task Name} & \textbf{Domain} & \textbf{Metric} & \textbf{Video Prompt} & \textbf{Image Prompt} & \textbf{Eval Prompt} \\
\midrule
\multicolumn{6}{l}{\textit{\textbf{Abstract Reasoning}}} \\
Maze & Abstract & Finish Task & \autoref{sec:maze_video_prompt} & \autoref{sec:maze_image_prompt} & \autoref{sec:maze_eval} \\
Sudoku & Abstract & Valid Solution & \autoref{sec:sudoku_video_prompt} & \autoref{sec:sudoku_image_prompt} & \autoref{sec:sudoku_eval} \\
ARC-AGI & Abstract & Valid Solution & \autoref{sec:arc_video_prompt} & \autoref{sec:arc_image_prompt} & \autoref{sec:arc_eval} \\
Math & Abstract & Valid Solution & \autoref{sec:math_video_prompt} & \autoref{sec:math_image_prompt} & \autoref{sec:math_eval} \\
\midrule
\multicolumn{6}{l}{\textit{\textbf{Embodied Navigation}}} \\
Top-down View Navigation & Navigation & Reach Goal & \autoref{sec:topdown_video_prompt} & \autoref{sec:topdown_image_prompt} & \autoref{sec:topdown_eval} \\
3D Real-World Navigation & Navigation & Success & \autoref{sec:3dnav_video_prompt} & \autoref{sec:3dnav_image_prompt} & \autoref{sec:3dnav_eval} \\
Last-Mile Nav. (Ego-centric) & Navigation & Success & \autoref{sec:fpv_video_prompt} & \autoref{sec:fpv_image_prompt} & \autoref{sec:fpv_eval} \\
Simultaneous Localization and Generation & Navigation & Success & \autoref{sec:slag_video_prompt} & \autoref{sec:slag_image_prompt} & \autoref{sec:slag_eval} \\
\midrule
\multicolumn{6}{l}{\textit{\textbf{Physical Commonsense}}} \\
Physical Commonsense & Physics & Plausibility & \autoref{sec:physics_video_prompt} & \autoref{sec:physics_image_prompt} & \autoref{sec:physics_eval} \\
\bottomrule
\end{tabular}
\end{table*}

\section{Prompts}
\label{sec:prompt_index}

This section provides a comprehensive index to all task-specific prompts used in our benchmark. Each task includes three types of prompts: (1) \textit{Video Generation Prompt} for generating task videos, (2) \textit{Image Generation Prompt} for creating initial frames or reference images, and (3) \textit{Evaluation Prompt} for assessing model outputs. The table below maps each task to its corresponding prompt sections in this appendix.

\clearpage
\onecolumn
\section{Released Prompt Templates}
\label{sec:released_prompt_templates}

For reproducibility, we provide the exact prompt templates implemented in our public repository\footnote{\url{https://github.com/mmgr-benchmark/video_reasoning_new}}. This section uses a single-column layout to faithfully render each template without line wrapping.

\subsection{Maze Solving (\texttt{benchmark/spatial/maze\_solving/generation\_prompts.py})}

\paragraph{Video Generation Prompt.}
\begin{center}
\begin{minipage}{0.95\textwidth}
\begin{promptlisting}
Create a 2D animation based on the provided image of a maze. The green square slides smoothly along the white path, stopping perfectly on the red square. The green square never slides or crosses into the black areas of the maze. The camera is a static, top-down view showing the entire maze. 

Maze:
- The maze paths are white, the walls are black.
- The green square moves to the goal position, represented by a red square.
- The green square slides smoothly along the white path.
- The green square never slides or crosses into the black areas of the maze.
- The green square stops perfectly on the red square.

Scene:
- No change in scene composition.
- No change in the layout of the maze.
- The green square travels along the white path without speeding up or slowing down.

Camera:
- Static camera.
- No zoom.
- No pan.
- No glitches, noise, or artifacts.
\end{promptlisting}
\end{minipage}
\end{center}

\paragraph{Image Generation Prompt.}
\begin{center}
\begin{minipage}{0.95\textwidth}
\begin{promptlisting}
Draw the maze showing the correct path from the green start square to the red goal square in a continuous blue line that stays within the white corridors and avoids the black walls.

Maze:
- The maze paths are white, the walls are black.
- The green square moves to the goal position, represented by a red square.
- The green square slides smoothly along the white path.
- The green square never slides or crosses into the black areas of the maze.
- The green square stops perfectly on the red square.
\end{promptlisting}
\end{minipage}
\end{center}

\subsection{Sudoku Solving (\texttt{benchmark/spatial/sudoku\_solving/generation\_prompts.py})}

\paragraph{Video Generation Prompt.}
\begin{center}
\begin{minipage}{0.95\textwidth}
\begin{promptlisting}
Create a static, smooth, animation that solves the given 4x4 or 9x9 Sudoku puzzle. Enter the missing numbers one by one with blue ink. Do not change anything else in the picture. Only fill the numbers in the empty cells so the Sudoku is solved properly.

Sudoku Rules:
- Sudoku is a logic-based number-placement puzzle.
- The grid is divided into rows, columns, and boxes (subgrids).
- Each row must contain all different numbers without repetition.
- Each column must contain all different numbers without repetition.
- Each box (subgrid) must contain all different numbers without repetition.
- For 4x4 puzzles: use numbers 1-4, with 2x2 boxes. Each row, column, and box sums to 10.
- For 9x9 puzzles: use numbers 1-9, with 3x3 boxes. Each row, column, and box sums to 45.

Scene:
- No change in scene composition.
- No change in the layout of the Sudoku grid.
- Numbers appear at a consistent pace.

Camera:
- Static camera.
- No zoom.
- No pan.
- No glitches, noise, or artifacts.
\end{promptlisting}
\end{minipage}
\end{center}

\paragraph{Image Generation Prompt.}
\begin{center}
\begin{minipage}{0.95\textwidth}
\begin{promptlisting}
Fill the Sudoku puzzle with the correct numbers in the empty cells with blue ink to solve the puzzle. Do not change anything else in the picture. Only fill the numbers in the empty cells so the Sudoku is solved properly.

Sudoku Rules:
- Sudoku is a logic-based number-placement puzzle.
- The grid is divided into rows, columns, and boxes (subgrids).
- Each row must contain all different numbers without repetition.
- Each column must contain all different numbers without repetition.
- Each box (subgrid) must contain all different numbers without repetition.
- For 4x4 puzzles: use numbers 1-4, with 2x2 boxes. Each row, column, and box sums to 10.
- For 9x9 puzzles: use numbers 1-9, with 3x3 boxes. Each row, column, and box sums to 45.
\end{promptlisting}
\end{minipage}
\end{center}

\subsection{Math Reasoning (\texttt{math\_data\_code/generation\_prompts.py})}

\paragraph{Video Generation Prompt.}
\begin{center}
\begin{minipage}{0.95\textwidth}
\begin{promptlisting}
Create a 2D animation using the provided image of a math problem, and solve it step by step.

Camera:
- Static camera.
- No zoom.
- No pan.
- No glitches, noise, or artifacts.
\end{promptlisting}
\end{minipage}
\end{center}

\paragraph{Image Generation Prompt.}
\begin{center}
\begin{minipage}{0.95\textwidth}
\begin{promptlisting}
Solve the math problem provided in the image step by step and write the solution in the image.
\end{promptlisting}
\end{minipage}
\end{center}

\subsection{ARC-AGI Video Prompt (\texttt{arc\_agi\_code/prompt.py})}

\paragraph{Video Generation Prompt.}
\begin{center}
\begin{minipage}{0.95\textwidth}
\begin{promptlisting}
Role
- You are a precise visual reasoner. You will receive a single composite image (the ONLY image input).
- That composite image contains the entire problem specification.

Composite Image Layout (read carefully)
- A thick horizontal RED separator divides the image into TWO parts: 1. ABOVE the red line: EXAMPLES - one or more rows. Each row has two tiles: LEFT=Input grid, RIGHT=Output grid. 2. BELOW the red line: TEST - exactly ONE row. LEFT=Test Input grid. RIGHT=an EMPTY red-outlined "ANSWER PANEL".
- Background is black, grid lines are white, colors use the ARC palette. Do NOT modify anything outside the answer panel.

Your Goal
- Infer the deterministic transformation that maps from input to output in EVERY training example.
- Apply the SAME transformation to the test input grid.
- Render ONLY the predicted test output INSIDE the red-outlined answer panel (the right tile of the test row).
- Everywhere else (all example tiles, the separator, and the test input tile) must remain PIXEL-IDENTICAL to the provided image.

Color & Rendering Constraints (ARC)
- Use the exact palette as seen in the image (sample from the provided image; DO NOT invent new colors):
  0: black, 1: blue, 2: red, 3: green, 4: yellow, 5: grey, 6: fuschia, 7: orange, 8: teal, 9: brown.
- Preserve the white grid lines and black background; do not paint over grid lines.
- Snap to the answer panel's grid cells; each filled cell is a solid, uniform color.
- Absolutely no antialiasing, feathering, gradients, glow, blending, or motion blur. Nearest-neighbor behavior only.

Video Behavior (for evaluation compatibility)
- One continuous shot. Static camera. No zooms, pans, cuts, transitions, overlays, captions, watermarks, or UI elements.
- Generation with the following phases:
  1) Stable context (~0.5s): Show the unmodified composite image.
  2) Reasoned drawing : Fill the answer panel ONLY, cell-by-cell in a clear row-major order.
     - All edits must occur strictly inside the red answer panel.
     - OPTIONAL: a subtle cursor/pen can be shown inside the panel; it must never leave the panel.
  3) Final freeze (>=0.5s): Hold the fully completed answer. Nothing moves.
- The LAST frames constitute the prediction to be graded; they must be perfectly still.

Rule Consistency & Causality
- The predicted output MUST satisfy the SAME rule observed across ALL training example pair(s) above the red line.
- Prefer the simplest consistent rule; if multiple rules fit, choose the one consistent with every example.
- If the learned rule implies an output grid shape different from the test input, conform to the answer panel' s tile (it is sized for the correct output). Fill it completely without crossing its border.

Hard Requirements (must follow)
- Modify pixels ONLY inside the red-outlined answer panel in the test row.
- Keep every other pixel in the image IDENTICAL to the input across the ENTIRE video.
- Do NOT introduce text, numbers, logos, arrows, highlights, masks, or any new marks outside the panel.
- Keep colors exact; no hue shifts or banding.
- No hallucinated content; no changes to example rows; the red separator remains unchanged.

Output Target
- Produce a short video where the ONLY difference between the first and the final frame is that the answer panel now contains the predicted output grid generated by applying the inferred rule to the test input.
- The final frame must be a clean, sharp, static image suitable for automated evaluation.

(You will be conditioned on exactly ONE composite image; use it as the immutable background and draw the solution strictly within the red answer panel in the test row.)
\end{promptlisting}
\end{minipage}
\end{center}

\subsection{Panoramic View Last-Mile Navigation}

\paragraph{Video Generation Prompt.}\label{sec:prompt_embodied_pano_video_gen}
\begin{center}
\begin{minipage}{0.95\textwidth}
\begin{promptlisting}
We provide four prompt variants tailored to different navigation scenarios:
Variant 1: COLOR_FLOOR01 (Single-floor navigation to red target)
Create a video showing a robot's "last mile" navigation within a 360-degree panoramic scene, filmed from a following, third-person perspective.
Scene & Environment:
- The environment is a static, photorealistic, 360-degree panoramic 3D scene (like the provided image).
- The scene contains static obstacles (furniture, walls) and a clear, navigable floor.
- The environment and all objects within it (except the robot) are completely static.
Agent & Goal:
- Agent (Start Point): A humanoid robot, visible in the frame.
- Goal (Destination): A bright red (#ff0000) target area clearly marked on the floor, visible in the distance.
Rules of Movement & Visibility:
- The robot moves with a natural, bipedal walking gait toward the destination.
- The robot maintains a steady, consistent walking speed.
- The robot performs a short, direct "last mile" approach, moving purposefully toward the red area.
- The task concludes when the robot stops walking and stands on or next to the red target area.
Camera:
- Perspective: The video is shown from a third-person, "over-the-shoulder" following view. The camera is positioned slightly behind and above the robot.
- Camera Motion: The camera moves smoothly with the robot, maintaining a stable distance and orientation. It pans and tilts as needed to keep both the robot (in the foreground) and the red target area (in the background) in the frame.
- Scene Motion: The view of the scene updates realistically as the camera moves through the 3D space, following the agent.
- Video Quality: The video feed is clear, well-lit, photorealistic, and free of glitches, sensor noise, or digital artifacts.
Variant 2: COLOR_FLOOR02PLUS (Multi-floor navigation with stairs to red target)
Create a video showing a robot's "last mile" navigation within a 360-degree panoramic scene, filmed from a following, third-person perspective. The navigation may span multiple stacked floors connected by staircases or ramps.
Scene & Environment:
- The environment is a static, photorealistic, 360-degree panoramic 3D scene (like the provided image).
- The scene contains static obstacles (furniture, walls) and a clear, navigable floor on every visible level.
- Multi-Level Layout: Show every traversed floor simultaneously, keeping the cutaway framing wide enough to reveal how the floors connect.
- The environment and all objects within it (except the robot) are completely static.
Agent & Goal:
- Agent (Start Point): A humanoid robot, visible in the frame.
- Goal (Destination): A bright red (#ff0000) target area clearly marked on the destination floor; never move or recolor it.
Rules of Movement & Visibility:
- The robot moves with a natural, bipedal walking gait toward the destination.
- The robot maintains a steady, consistent walking speed.
- Stair Navigation: When changing floors, the robot climbs or descends one step at a time with planted feet---no teleporting, sliding, or clipping.
- The robot performs a purposeful, efficient approach toward the red area.
- The task concludes when the robot stops walking and stands fully inside the red target area.
Camera:
- Perspective: The video is shown from a third-person, "over-the-shoulder" following view. Keep both the robot and the red goal visible, even when they occupy different levels.
- Camera Motion: The camera moves smoothly with the robot, adjusting height as needed to keep the robot centered while still revealing the overall multi-floor layout.
- Scene Motion: Only the robot moves; walls, furniture, and the red target remain static.
- Video Quality: The video feed is clear, well-lit, photorealistic, and free of glitches, sensor noise, or digital artifacts.
Variant 3: OBJECT_FLOOR01 (Single-floor navigation to described location)
Create a video showing a robot's "last mile" navigation within a 360-degree panoramic scene, filmed from a following, third-person perspective.
Scene & Environment:
- The environment is a static, photorealistic, 360-degree panoramic 3D scene (like the provided image).
- The scene contains static obstacles (furniture, walls) and a clear, navigable floor.
- The environment and all objects within it (except the robot) are completely static.
Agent & Goal:
- Agent (Start Point): A humanoid robot, visible in the frame.
- Goal (Destination): A location described as: "<LOCATION_DESCRIPTION>" --- keep the destination exactly as shown originally; do not add bright red markers or any other artificial overlays.
Rules of Movement & Visibility:
- The robot moves with a natural, bipedal walking gait toward the described location.
- The robot maintains a steady, consistent walking speed.
- The robot performs a short, direct "last mile" approach, moving purposefully toward the described destination.
- The task concludes when the robot stops walking and stands on or next to the location that matches the description.
Camera:
- Perspective: The video is shown from a third-person, "over-the-shoulder" following view. The camera is positioned slightly behind and above the robot.
- Camera Motion: The camera moves smoothly with the robot, maintaining a stable distance and orientation. It pans and tilts as needed to keep both the robot (in the foreground) and the described destination area (in the background) in the frame.
- Scene Motion: The view of the scene updates realistically as the camera moves through the 3D space, following the agent.
- Video Quality: The video feed is clear, well-lit, photorealistic, and free of glitches, sensor noise, or digital artifacts.
Variant 4: OBJECT_FLOOR02PLUS (Multi-floor navigation to described location)
Create a video showing a robot's "last mile" navigation within a 360-degree panoramic scene, filmed from a following, third-person perspective. The navigation may span multiple stacked floors connected by staircases or ramps.
Scene & Environment:
- The environment is a static, photorealistic, 360-degree panoramic 3D scene (like the provided image).
- The scene contains static obstacles (furniture, walls) and a clear, navigable floor on every visible level.
- Multi-Level Layout: Show every traversed floor simultaneously, keeping the cutaway framing wide enough to reveal how the floors connect.
- The environment and all objects within it (except the robot) are completely static.
Agent & Goal:
- Agent (Start Point): A humanoid robot, visible in the frame.
- Goal (Destination): A location described as: "<LOCATION_DESCRIPTION>" --- preserve the existing look of that destination and never replace it with a red marker or highlight.
Rules of Movement & Visibility:
- The robot moves with a natural, bipedal walking gait toward the described destination.
- The robot maintains a steady, consistent walking speed.
- Stair Navigation: When changing floors, the robot climbs or descends one step at a time with planted feet---no teleporting, sliding, or clipping.
- The robot performs a purposeful, efficient approach toward the described area.
- The task concludes when the robot stops walking and stands fully inside or immediately beside the location that matches the description.
Camera:
- Perspective: The video is shown from a third-person, "over-the-shoulder" following view. Keep both the robot and the described goal visible, even when they occupy different levels.
- Camera Motion: The camera moves smoothly with the robot, adjusting height as needed to keep the robot centered while still revealing the overall multi-floor layout.
- Scene Motion: Only the robot moves; walls, furniture, and the described destination remain static.
- Video Quality: The video feed is clear, well-lit, photorealistic, and free of glitches, sensor noise, or digital artifacts.
\end{promptlisting}
\end{minipage}
\end{center}

\paragraph{Image Generation Prompt.}\label{sec:prompt_embodied_pano_image_gen}
\begin{center}
\begin{minipage}{0.95\textwidth}
\begin{promptlisting}
We provide four prompt variants tailored to different navigation scenarios:
Variant 1: COLOR_FLOOR01 (Single-floor navigation to red target)
Create a single photorealistic image (or edit the provided panoramic frame) that captures the final state of a humanoid robot completing its "last mile" navigation inside a 360-degree indoor environment.
Scene & Environment:
- Use the provided 360-degree panorama as the base plate. Preserve all lighting, materials, and geometry exactly as they appear in the original reference.
- The scene contains static obstacles (furniture, walls) and a navigable floor; nothing in the environment is moving.
- If you add shadows or reflections for the robot, match the existing light directions.
Agent & Goal Status:
- Agent: Identify the humanoid robot already present in the input image, remove it cleanly from its starting spot, and relocate the same robot asset to its final position.
- Goal (Destination): A bright red (#ff0000) target area painted on the floor, already present in the scene.
- Depict the robot standing firmly on or immediately beside the red target, conveying that the destination has been reached. Do not recolor or relocate the red area.
- Draw a bright green (#00ff00) trajectory line that traces the robot's path from the original position to the destination.
- After relocating the robot, revise the original starting area so only natural floor detail (and any markers that already existed) remain-no duplicate robot silhouettes.
Image Requirements:
- Present the moment after the robot has stopped; no motion blur, trails, or animation cues.
- Keep the framing similar to an over-the-shoulder third-person view, slightly behind and above the robot so both the robot and the red target remain clear.
- Ensure the final render/edit is crisp, well lit, and free from artifacts. The only modifications should communicate the robot's successful arrival.
Variant 2: COLOR_FLOOR02PLUS (Multi-floor navigation to red target)
Create a single photorealistic image (or edit the provided panoramic frame) that captures the final state of a humanoid robot completing its "last mile" navigation across stacked floors connected by stairs or ramps.
Scene & Environment:
- Use the referenced multi-level panorama as the base. Maintain the cutaway layout so every traversed floor and its connections remain visible.
- All architectural elements, furniture, and props stay frozen in place; only the robot's final pose may be modified or inserted.
- Lighting continuity with the source panorama is essential-shadows, reflections, and highlights must align.
Agent and Goal Status:
- Agent: Locate the humanoid robot already visible in the reference, remove it from the start pose, and reinsert it at the final location on the destination floor.
- Goal (Destination): A bright red (#ff0000) target region on the destination floor. Keep it exactly where and how it appears in the original data.
- Portray the robot standing fully inside the red area (or touching its edge) to emphasize that the destination has been achieved.
- Render a continuous bright green (#00ff00) trajectory line that follows the robot's travel route, including the climb/descent between floors.
- Clean up the original starting area so that only the untouched floor (and any static markers) remain, with no leftover robot ghosting.
Image Requirements:
- The image is a single, clean frame-no sequential panels or motion cues.
- Camera viewpoint mirrors a following third-person angle that simultaneously reveals the robot and the multi-floor context.
- The final output should feel like a high-fidelity still pulled from the end of a navigation recording.
Variant 3: OBJECT_FLOOR01 (Single-floor navigation to described location)
Create a single photorealistic image (or edit the provided panoramic frame) that captures the final state of a humanoid robot completing its "last mile" navigation within a 360-degree indoor environment.
Scene & Environment:
- Start from the supplied panorama and keep every background detail untouched aside from the robot placement.
- The world is static and matches the real furniture, walls, and lighting of the reference scene.
Agent & Goal Status:
- Agent: Identify the humanoid robot in the panorama, remove it from its starting pose, and reposition the same robot asset at the destination.
- Goal (Destination): A location described as: **"<LOCATION_DESCRIPTION>"**. Depict the exact object/area from the description without adding artificial highlights.
- Show the robot standing on, holding, or immediately beside that described location to prove the navigation succeeded.
- Add a bright green (#00ff00) trajectory line showing the precise route from the starting spot to the described goal while respecting the existing floor layout.
- Once the robot has been moved, restore the starting area so it no longer contains the old robot placement-only the ambient scene details remain.
Image Requirements:
- Frame the scene from an over-the-shoulder third-person angle so both the robot and the described target are clearly readable.
- Avoid depicting motion; the robot should look stable, with grounded feet and relaxed posture.
- Maintain photorealistic lighting and detail fidelity consistent with the panorama.
Variant 4: OBJECT_FLOOR02PLUS (Multi-floor navigation to described location)
Create a single photorealistic image (or edit the provided panoramic frame) that captures the final state of a humanoid robot completing its "last mile" navigation across multiple vertically stacked floors.
Scene & Environment:
- Use the given multi-floor panorama as the base plate; ensure the relationships between floors, staircases, or ramps remain accurate.
- Keep every environmental element immutable except for the robot and any subtle contact cues needed to show arrival.
Agent & Goal Status:
- Agent: Detect the humanoid robot present in the scene, remove it from the initial pose, and place the same asset at the described destination on the correct floor.
- Goal (Destination): A location described as: **"<LOCATION_DESCRIPTION>"**. Reproduce that exact object/area without overlays or color changes.
- Depict the robot positioned inside or directly adjacent to the described destination zone so the successful completion is unmistakable.
- Draw a bright green (#00ff00) trajectory that winds through every relevant floor and bridges stair transitions, clearly illustrating how the agent reached the goal.
- After relocation, touch up the initial robot position so it blends back into the untouched environment.
Image Requirements:
- Compose the still image from a third-person viewpoint that lets the viewer see both the robot and the relevant floors at once.
- Convey a finished moment-no motion blur, repeated frames, or animation hints.
- Preserve the realism of the panorama; edits should be seamless, noise-free, and physically plausible.
\end{promptlisting}
\end{minipage}
\end{center}

\paragraph{Video Evaluation Prompt.}\label{sec:prompt_embodied_pano_video_eval}
\begin{center}
\begin{minipage}{0.95\textwidth}
\begin{promptlisting}
You are an expert evaluator for task01 (Last-Mile Navigation, panoramic FPV). Judge whether the humanoid robot in the generated video correctly approaches its designated destination (either a bright red target patch or a described object) while preserving physical realism, instruction fidelity, and scene consistency.

SCENE & INPUTS
- INITIAL_PANORAMA: a static, photorealistic 360° panorama that shows the robot’s starting pose (its back centered in the frame) and the surrounding environment. Obstacles (walls, furniture) are fixed and immovable.
- DESTINATION_REFERENCE:
    • For color levels: a bright red (#ff0000) floor patch is visible in the initial panorama.
    • For object levels: a separate location description text specifies the destination (e.g., “stand next to the wooden cabinet on the right”). This description replaces the red patch as the authoritative goal cue.
- NAVIGATION_VIDEO: a first-person-style rendering where each new frame is a physically plausible continuation of the previous view (no brand-new environments, just viewpoint progression along the robot’s path).

ENVIRONMENT & MOTION RULES
- The robot must walk with a natural, bipedal gait at a steady pace, executing a short “last mile” approach toward the referenced destination (red patch or described object/spot).
- It must remain within traversable floor space, respecting all static obstacles.
- The trial ends once the robot stops on or right next to the specified destination.

GENERAL DIRECTIONS
- Treat the initial panorama plus any provided location description as ground truth for both the starting state and the target’s appearance/location. The video’s opening frames must match this reference.
- Always compare the final destination to BOTH the initial panorama and any accompanying textual description; any mismatch in position, appearance, or semantics means DESTINATION_INTEGRITY_SCORE = 0.
- Watch the entire video carefully. If any metric is ambiguous, assign 0 (fail-safe).
- All metrics are binary. Physical violations (teleports, collisions, floating) or scene edits (new furniture appearing) must be penalized even if the agent reaches the target.

METRICS
1. SUCCESS_SCORE_3D – 1 if the robot reaches and stops on/next to the specified destination (red patch or described object/location) by the end of the video; else 0.
2. ORACLE_SUCCESS_SCORE_3D – 1 if the trajectory ever passes through or pauses inside the correct destination region even if it does not finish there; else 0.
3. OBJECT_SEMANTIC_SCORE – 1 if no collisions or phasing through walls/furniture; else 0.
4. AGENT_CONSISTENCY_SCORE – 1 if motion is temporally continuous with no teleporting, pose pops, or size jumps; else 0.
5. SPATIAL_ALIGNMENT_SCORE – 1 if heading, walking direction, and elevation changes stay coherent (turn then move, no backward glide, no floating between floors); else 0.
6. DESTINATION_INTEGRITY_SCORE – 1 if the observed destination in the video matches the initial panorama/red patch or the textual description (same placement, appearance, semantics) AND the robot finishes within/on that unchanged goal; 0 if any noticeable difference or if the robot stops elsewhere.
7. SCENE_CHANGE_SCORE – 1 if the panoramic environment stays static (no new objects/lighting shifts beyond expected view changes); else 0.

EVALUATION STEPS
1. Verify the opening frames align with the initial panorama (robot back centered, same obstacles, same destination cues).
2. Track the robot’s trajectory toward the referenced destination, noting whether it ever enters or finishes on the correct target.
3. Inspect for collisions, clipping, teleportation, or unnatural speed/pose shifts.
4. Confirm heading/elevation coherence as camera perspectives update along the walk.
5. Compare the final target appearance with the initial reference and description; any discrepancy immediately zeroes DESTINATION_INTEGRITY_SCORE.
6. Ensure the broader scene stays identical aside from expected viewpoint changes.
7. Assign binary scores for each metric using the strict definitions above.

OUTPUT FORMAT
Return ONLY a JSON object with two top-level fields:
1. "SCORES": matches the task03_evaluation_output_format.txt schema, using string values "0" or "1".
2. "REASONING": mirrors every metric key; provide a concise sentence citing visual evidence for each score.

Structure example:
{
  "SCORES": {
    "SUCCESS_SCORE_3D": "<0 or 1>",
    "ORACLE_SUCCESS_SCORE_3D": "<0 or 1>",
    "OBJECT_SEMANTIC_SCORE": "<0 or 1>",
    "AGENT_CONSISTENCY_SCORE": "<0 or 1>",
    "SPATIAL_ALIGNMENT_SCORE": "<0 or 1>",
    "DESTINATION_INTEGRITY_SCORE": "<0 or 1>",
    "SCENE_CHANGE_SCORE": "<0 or 1>"
  },
  "REASONING": {
    "SUCCESS_SCORE_3D": "<brief justification>",
    "ORACLE_SUCCESS_SCORE_3D": "<brief justification>",
    "OBJECT_SEMANTIC_SCORE": "<brief justification>",
    "AGENT_CONSISTENCY_SCORE": "<brief justification>",
    "SPATIAL_ALIGNMENT_SCORE": "<brief justification>",
    "DESTINATION_INTEGRITY_SCORE": "<brief justification>",
    "SCENE_CHANGE_SCORE": "<brief justification>"
  }
}
No extra commentary outside this JSON object.
\end{promptlisting}
\end{minipage}
\end{center}

\subsection{Top-Down View Real-World Navigation}

\paragraph{Video Generation Prompt.}\label{sec:prompt_embodied_2d_video_gen}
\begin{center}
\begin{minipage}{0.95\textwidth}
\begin{promptlisting}
Create a video showing an agent navigating a 2D top-down environment from a starting point to a target destination.
Scene & Environment:
- The environment is a static 2D top-down floor plan (e.g., a maze or office layout).
- The scene has two distinct types of areas: navigable paths (e.g., white) and non-navigable obstacles/walls (e.g., black).
- The layout of the environment is completely static throughout the video.
- Multi-Level Layouts: If there are two or more stacked floors, depict each as its own 2D map panel arranged from the highest floor at the top down to the lowest floor so that "up-to-down" clearly reads as moving from upper levels to lower levels.
Agent & Goal:
- Agent: A realistic robot (top-down view, matching the unitree-g1-humanoid-robotic-topview).
- Start Point: The robot begins positioned perfectly on a bright blue (#0000ff) triangular starting marker.
- Agent Orientation: The "front" of the robot (the side without the black panel) must be aligned with the single, pointed vertex of the blue triangle marker. This vertex indicates the agent's initial "facial direction."
- Goal (Destination): A bright red (#ff0000) target area clearly marked on the floor plan.
- Static Markers: The blue triangle and red goal are static references that never move; only the robot changes position while the green trajectory records its motion.
Rules of Movement & Visibility:
- The robot agent is the only object that moves. The blue triangle marker is static; it marks the origin and does not move for the entire video.
- The robot agent slides smoothly along the navigable paths, starting from the blue triangle marker. It does not teleport.
- The robot maintains a steady, consistent speed throughout the navigation.
- Agent Rotation: As the agent moves, it rotates realistically to face its direction of travel. Its "front" should always point forward along its immediate path. It should not slide sideways or backward.
- The agent obeys physical constraints: it cannot clip through, cross, or move into non-navigable walls or obstacles.
- The agent moves purposefully and efficiently toward the red region, finding a plausible path around obstacles.
- Vertical Transitions: When the agent uses stairs/ramps to go upstairs or downstairs, its position should jump between the floor panels; the bright green (#00ff00) trajectory briefly breaks or discretely bridges between the maps before resuming on the destination floor.
- Trajectory: As the robot agent moves, it leaves a permanent, bright green (#00ff00) trajectory line tracing its exact path from the start point.
- Goal Persistence: The task concludes when the robot agent stops perfectly on the red target region. The red region must remain visible and is not erased or fully occluded by the agent.
Camera:
- Perspective: The video is shown from a single, static, top-down view that shows the entire environment.
- Camera Motion: The camera does not move, pan, zoom, or rotate. Its position is fixed.
- Scene Motion: The robot agent is the only moving object in the video. The blue triangle marker, red target, and all parts of the environment are static. The green trajectory line is drawn progressively as the agent moves.
- Video Quality: The video feed is clear, 2D, and free of glitches, noise, or artifacts.
\end{promptlisting}
\end{minipage}
\end{center}

\paragraph{Image Generation Prompt.}\label{sec:prompt_embodied_2d_image_gen}
\begin{center}
\begin{minipage}{0.95\textwidth}
\begin{promptlisting}
We provide four prompt variants tailored to different navigation scenarios:
Variant 1: COLOR_FLOOR01 (Single-floor navigation to red target)
Create a single high-resolution still image (or edit the provided floor-plan frame) that captures the final moment of a robot completing its 2D top-down navigation on a single-floor map.
Scene & Environment:
- Use the supplied static 2D map exactly as rendered in the reference image (maze, office, etc.). Do not redraw, re-color, or move the camera-the top-down orthographic view must stay fixed.
- Navigable paths remain light, non-navigable cells remain dark, and every wall/obstacle keeps the same geometry.
- Keep the bright blue (#0000ff) triangular starting marker exactly where it already exists. The triangle still shows the initial heading even though the robot has moved away.
Agent & Goal Status:
- Agent: A realistic top-view humanoid robot (match the provided unitree-g1 reference style).
- Goal: A bright red (#ff0000) destination patch that already exists in the scene.
- Depict the robot standing squarely on or immediately adjacent to the red patch to confirm the destination has been achieved. Preserve the red patch's color, position, and shape.
- Draw the entire bright green (#00ff00) trajectory line that records the exact path from the blue triangle to the red goal. The path should be continuous, obey the maze, and end beneath the robot's feet.
Image Requirements:
- The robot should appear at rest-no motion blur or repeated silhouettes.
- Align the robot's "front" (the side without the black panel) with its final facing direction. It should never appear sideways relative to the green path.
- Maintain crisp 2D rendering with clean edges and legible contrast between walkable space, walls, and markers.
Variant 2: COLOR_FLOOR02PLUS (Multi-floor navigation to red target)
Create a single high-resolution still image (or edit the provided multi-floor floor-plan frame) that captures the final moment of a robot completing its 2D top-down navigation across multiple stacked floors.
Scene & Environment:
- Use the existing multi-floor layout as-is. Each floor remains its own panel, stacked vertically from highest to lowest so viewers read motion from top to bottom.
- Keep every staircase/ramp connector exactly aligned between panels, and retain the original color palette (light paths, dark obstacles).
- The camera is an unmoving orthographic top view. Do not tilt, zoom, or rearrange the panels.
Agent & Goal Status:
- Agent: The same realistic top-view humanoid robot icon.
- Goal: A bright red destination patch located on one of the panels-keep the patch untouched.
- Show the robot fully inside the red goal on the correct floor panel to indicate the navigation is over.
- Render a bright green trajectory that traces the full path, including any vertical transitions. When crossing panels, bridge the path with a short dashed or kinked segment that connects the relevant stair locations so the viewer can follow the route at a glance.
Image Requirements:
- Only the final state is depicted. The robot stands still, and the red + blue markers remain static reference points.
- The robot's heading should match the final segment of the trajectory.
- Ensure every panel stays legible and evenly lit, as if the still was captured from the last frame of the original animation.
Variant 3: OBJECT\_FLOOR01 (Single-floor navigation to described location)
Create a single high-resolution still image (or edit the provided floor-plan frame) that captures the final moment of a robot completing its 2D top-down navigation on a single-floor map toward a location described as: **"<LOCATION_DESCRIPTION>"**.
Scene & Environment:
- Preserve the exact layout, coloring, and fixed top-down camera of the provided map. Do not introduce new highlights or overlays on the destination; rely on the natural appearance of the described area.
- Keep the bright blue (#0000ff) triangular start marker untouched at its original coordinates.
Agent & Goal Status:
- Agent: A realistic top-view humanoid robot styled like the unitree-g1 reference.
- Goal: The precise region/object described in **"<LOCATION_DESCRIPTION>"**. Do not recolor it or replace it with a red patch.
- Position the robot directly atop or immediately beside that described location to prove the navigation succeeded.
- Draw a bright green (#00ff00) trajectory line from the blue triangle to the destination, respecting walls and obstacles.
Image Requirements:
- Show the robot standing still with its front aligned to the final travel direction.
- Avoid motion cues; the still should feel like the last frame of a navigation video.
- Maintain sharp 2D rendering, consistent lighting, and clean separation between walkable and blocked cells.
Variant 4: OBJECT_FLOOR02PLUS (Multi-floor navigation to described location)
Create a single high-resolution still image (or edit the provided multi-floor frame) that captures the final moment of a robot completing its 2D top-down navigation toward a location described as: **"<LOCATION_DESCRIPTION>"** across multiple stacked floors.
Scene & Environment:
- Retain the original panel arrangement (top panel = highest floor). Keep every architectural detail and connector exactly where it appears in the source image.
- The entire scene stays in a fixed orthographic top-down view. No camera motion, parallax, or re-layering is permitted.
Agent & Goal Status:
- Agent: The same realistic top-view humanoid robot icon.
- Goal: The specific location described in **"<LOCATION_DESCRIPTION>"** on the correct floor panel.
- Depict the robot resting on or immediately next to that described feature without inventing new highlights. If you need to emphasize it, rely on precise placement and the green trajectory rather than extra markers.
- Draw the bright green (#00ff00) path across every floor in the traversal. Bridge floors at the staircase/ramp connectors with subtle dashed segments so viewers can follow the entire route.
Image Requirements:
- The still image represents the final state only; nothing implies ongoing motion.
- The robot's heading should align with the last step it took before stopping.
- Multi-floor panels must remain crisp, evenly spaced, and easy to read, matching the palette of the original reference.
\paragraph{Video Evaluation Prompt.}\label{sec:prompt_embodied_2d_video_eval}
You are an expert evaluator for 2D top-down navigation rollouts. Judge whether the agent depicted in the generated video satisfies the navigation goal while preserving planar physical realism and strict instruction fidelity.

INPUTS YOU RECEIVE
1. INITIAL_IMAGE – a single top-down RGB frame that shows the agent’s starting cell, orientation, and surrounding obstacles.
2. LOCATION_DESCRIPTION(OPTIONAL) – a textual destination description provided only for hard “object” levels; otherwise this field may be empty or “NONE”.
3. NAVIGATION_VIDEO – a video generated by a model such as VEO3 or Sora2 that shows the entire navigation attempt from a 2D bird’s-eye view.

GENERAL DIRECTIONS
- Treat the initial image as the authoritative starting state. Verify that the video begins consistently with this frame (agent pose, visible tiles, obstacle layout).
- Use the location description to pin down the correct destination semantics (object identity, coordinates, relative placement). When no description is given, infer the intended goal from markers visible in the initial image plus the agent’s behavior.
- Watch the whole video carefully. If there is any ambiguity about collisions, teleports, or map edits, assume the stricter (failing) interpretation and set the relevant metric to 0.
- Each metric is binary (0 or 1). Record 0 whenever evidence is missing, unclear, or contradicts the pass condition.
- The agent must obey planar physics: move through traversable cells only, never clip through walls, and maintain temporally continuous motion.
- If more than one agent/avatar moves in the video, judge SUCCESS/DESTINATION/SCENE/CONSISTENCY/SPATIAL/OBJECT metrics only when **all** agents satisfy the requirement. ORACLE success, however, is satisfied if **any single agent** passes near the destination at least once.

METRICS (REFERENCE THE TASK02 CRITERIA FILE)

1. SUCCESS_SCORE_2D
   - 1 if every moving agent reaches the designated 2D goal footprint and halts inside it by the end of the video.
   - 0 if any agent never reaches, overshoots, keeps moving after arrival, or the destination cannot be confirmed.

2. ORACLE_SUCCESS_SCORE_2D
   - 1 if, at any point, at least one agent’s path passes through or immediately adjacent to the correct goal region even if no one stops there permanently.
   - 0 if no agent ever enters or brushes past the destination vicinity.

3. OBJECT_SEMANTIC_SCORE
   - 1 if no agent collides with or phases through solid obstacles such as walls, furniture, or blocked tiles.
   - 0 if any agent exhibits overlap, clipping, or impossible interaction.

4. AGENT_CONSISTENCY_SCORE
   - 1 if every agent’s icon, position, and orientation evolve smoothly without teleportation, scale jumps, or sudden resets.
   - 0 if any agent shows temporal discontinuity or impossible acceleration.

5. SPATIAL_ALIGNMENT_SCORE
   - 1 if each agent’s heading (if shown) matches its displacement direction and rotations are smooth on the 2D plane.
   - 0 if any agent slides sideways, moves opposite its facing direction, or otherwise violates planar motion logic.

6. DESTINATION_INTEGRITY_SCORE
   - 1 if the destination shown in the video matches the initial specification (visual goal in the initial image and/or the textual location description) AND every agent finishes inside that unchanged region.
   - 0 if the destination is moved, resized, recolored, swapped, contradicts the text description, or any agent stops outside the intact region.

7. SCENE_CHANGE_SCORE
   - 1 if the map layout, lighting, and object placements remain static aside from expected parallax.
   - 0 if any scene element is added, removed, or morphs during the video (including agent-induced edits).

EVALUATION STEPS
1. Compare the initial image with the video’s opening frames to confirm continuity.
2. Identify the goal location using the description (if any) and visual cues.
3. Observe the entire trajectory for success proximity, collisions, teleportation, and spatial alignment violations.
4. Inspect the goal region for tampering or relocation by comparing the final destination to BOTH the initial image and the location description. Any mismatch sets DESTINATION_INTEGRITY_SCORE to 0, even if the agent stops there.
5. Note any scene-wide changes between frames.
6. Assign each metric a binary score based strictly on the definitions above.

OUTPUT FORMAT
Return ONLY a JSON object with two top-level sections:
1. "SCORES" – matches the exact metric format in task02_evaluation_output_format.txt (string values "0" or "1").
2. "REASONING" – a dictionary mirroring the metric keys; each value is a short sentence explaining why the corresponding score is 0 or 1 (cite concrete visual evidence).

Example schema:
{
  "SCORES": {
    "SUCCESS_SCORE_2D": "<0 or 1>",
    "ORACLE_SUCCESS_SCORE_2D": "<0 or 1>",
    "OBJECT_SEMANTIC_SCORE": "<0 or 1>",
    "AGENT_CONSISTENCY_SCORE": "<0 or 1>",
    "SPATIAL_ALIGNMENT_SCORE": "<0 or 1>",
    "DESTINATION_INTEGRITY_SCORE": "<0 or 1>",
    "SCENE_CHANGE_SCORE": "<0 or 1>"
  },
  "REASONING": {
    "SUCCESS_SCORE_2D": "<brief justification>",
    "ORACLE_SUCCESS_SCORE_2D": "<brief justification>",
    "OBJECT_SEMANTIC_SCORE": "<brief justification>",
    "AGENT_CONSISTENCY_SCORE": "<brief justification>",
    "SPATIAL_ALIGNMENT_SCORE": "<brief justification>",
    "DESTINATION_INTEGRITY_SCORE": "<brief justification>",
    "SCENE_CHANGE_SCORE": "<brief justification>"
  }
}
Do not include any other text outside this JSON object.
% \paragraph{Evaluation Results}
\end{promptlisting}
\end{minipage}
\end{center}

\subsection{3D Real-World Navigation}

\paragraph{Video Generation Prompt.}\label{sec:prompt_embodied_3d_video_gen}
\begin{center}
\begin{minipage}{0.95\textwidth}
\begin{promptlisting}
We provide four prompt variants tailored to different navigation scenarios:
Variant 1: COLOR_FLOOR01 (Single-floor navigation to red target)
Create a video showing a humanoid robot successfully navigating from a starting point through a 3D indoor environment to reach a specific target destination. The video should be from a fixed, external viewpoint.
Scene & Environment:
- The environment is a photorealistic, 3D indoor space, shown in a "cutaway" or "dollhouse" style.
- The scene contains standard static obstacles like walls, furniture (desks, chairs, couches), and doorways.
- The environment and all objects within it (except the robot) are completely static.
- The floor is flat and provides the only navigable surface.
- Preserve the existing scene layout, lighting, and furnishing exactly as provided; do not introduce, remove, or rearrange any elements.
- Destination Integrity: Do not change the size, color, or placement of the red goal area relative to the provided scene.
Agent & Goal:
- Agent: A clearly mechanical humanoid robot (silver or white body panels, visible joints, illuminated visor/sensors) standing roughly 1.5-2 meters tall; it must look robotic, never human.
- Start Point: The robot begins standing at the designated starting location on the floor.
- Agent Orientation: The robot's "front" (facial direction) must be aligned with the specified initial heading indicated in the scene.
- Goal (Destination): A bright red (#ff0000) region clearly marked on the floor; render it exactly where it already exists in the scene.
Rules of Movement & Visibility:
- The robot moves with a natural, bipedal walking gait. It does not slide, float, or teleport.
- The robot maintains a steady, consistent walking speed throughout the navigation.
- The robot obeys physical constraints: it cannot clip through or pass through solid objects.
- The robot must actively navigate around obstacles by finding a clear, plausible path.
- The robot moves purposefully and efficiently toward the red region.
- Static Markers: The designated start marker and the red target region are static markings on the floor. They do not move, fade, or disappear.
- The task concludes when the robot stops walking and stands with its feet fully inside the red target region.
- Wall Fading: If a wall or large obstacle is between the camera's fixed position and the robot, that obstacle must fade or become transparent to keep the robot fully visible at all times.
Camera:
- Perspective: The video is shown from a single, static, third-person isometric view (a "dollhouse" view).
- Camera Motion: The camera does not move, pan, zoom, or rotate. Its position is fixed for the entire video.
- Scene Motion: The humanoid robot is the only object that moves in the entire video. All other elements (furniture, walls, the start marker, the red target) are completely static.
- Video Quality: The video feed is clear, well-lit, photorealistic, and free of glitches, sensor noise, or digital artifacts.
Variant 2: COLOR_FLOOR02PLUS (Multi-floor navigation to red target)
Create a video showing a humanoid robot successfully navigating from a starting point through a multi-level 3D indoor environment to reach a specific target destination. The video should be from a fixed, external viewpoint.
Scene & Environment:
- The environment is a photorealistic, multi-story indoor space shown in a "cutaway" or "dollhouse" style.
- A clearly modeled staircase connects the lower floor to at least one upper floor; this staircase is the only way to change elevations.
- The destination region may be located on an upper floor or a downstairs area, requiring the robot to ascend or descend the stairs mid-trajectory.
- The scene contains standard static obstacles like walls, furniture (desks, chairs, couches), doorways, and railings along the stairs.
- The environment and all objects within it (except the robot) are completely static.
- Preserve the existing scene layout, lighting, and furnishing exactly as provided; do not introduce, remove, or rearrange walls, furniture, or staircases.
- Destination Integrity: Keep the size, color, and placement of the red target area exactly as it already exists in the provided scene.
- Floors and stair treads are the only navigable surfaces; no elevators, ramps, or floating platforms are available.
Agent & Goal:
- Agent: A clearly mechanical humanoid robot (silver or white body panels, visible joints, illuminated visor/sensors) standing roughly 1.5-2 meters tall; it must look robotic, never human.
- Start Point: The robot begins standing at the designated starting location on the floor.
- Agent Orientation: The robot's "front" (facial direction) must be aligned with the specified initial heading indicated in the scene.
- Goal (Destination): A bright red (#ff0000) region clearly marked on the floor. Render and keep it exactly where it already exists in the scene.
Rules of Movement & Visibility:
- The robot moves with a natural, bipedal walking gait. It does not slide, float, or teleport.
- The robot maintains a steady, consistent walking speed throughout the navigation.
- The robot obeys physical constraints: it cannot clip through or pass through solid objects.
- Stair Navigation: When moving between floors, the robot climbs or descends the staircase step-by-step, keeping its feet planted on individual treads.
- The robot must actively navigate around obstacles by finding a clear, plausible path, including tight turns onto landings or upper-floor hallways.
- The robot moves purposefully and efficiently toward the red region, even if it is located upstairs.
- Static Markers: The designated start marker and the red target region are static markings on the floor. They do not move, fade, or disappear.
- The task concludes when the robot stops walking and stands with its feet fully inside the red target region.
- Wall Fading: If a wall or large obstacle is between the camera's fixed position and the robot, that obstacle must fade or become transparent to keep the robot fully visible at all times.
Camera:
- Perspective: The video is shown from a single, static, third-person isometric view (a "dollhouse" view).
- Camera Motion: The camera does not move, pan, zoom, or rotate. Its position is fixed for the entire video.
- Scene Motion: The humanoid robot is the only object that moves in the entire video. All other elements (furniture, walls, the start marker, the red target) are completely static.
- Video Quality: The video feed is clear, well-lit, photorealistic, and free of glitches, sensor noise, or digital artifacts.
Variant 3: OBJECT_FLOOR01 (Single-floor navigation to described location)
Create a video showing a humanoid robot successfully navigating from a starting point through a 3D indoor environment to reach a specific target destination.
Scene & Environment:
- The environment is a photorealistic, 3D indoor space, such as a modern office or apartment.
- The scene contains standard static obstacles like walls, furniture (desks, chairs, couches), and doorways.
- The environment is static: objects do not move, and doors are assumed to be open.
- The floor is flat and provides the only navigable surface.
- Preserve the existing scene layout, lighting, and furnishing exactly as provided; do not introduce, remove, or rearrange any elements.
Agent & Goal:
- Agent (Start Point): A clearly mechanical humanoid robot (silver or white body panels, visible joints, illuminated visor/sensors) standing roughly 1.5-2 meters tall; it must look robotic, never human.
- Goal (Destination): keep the destination area exactly as provided; do not enlarge, recolor, or move it.
Rules of Movement:
- The robot moves with a natural, bipedal walking gait. It does not slide, float, or teleport.
- The robot maintains a steady, consistent walking speed throughout the navigation.
- The robot obeys physical constraints: it cannot clip through or pass through solid objects (walls, furniture).
- The robot must actively navigate around obstacles by finding a clear, plausible path.
- The robot moves purposefully and efficiently toward the described location.
- The task concludes when the robot stops walking, having clearly arrived at the location that matches the destination description.
Camera:
- The video is shown from a first-person point-of-view (POV), simulating the robot's vision.
- The camera is mounted at the robot's eye level.
- The camera view moves smoothly as the robot walks forward and turns its body.
- The view is stable: no excessive head-bobbing, jitter, or motion blur that would be unnatural for a robotic sensor.
- The video feed is clear, well-lit, and photorealistic.
- There are no glitches, sensor noise, or digital artifacts in the video.
Variant 4: OBJECT_FLOOR02PLUS (Multi-floor navigation to described location)
Create a video showing a humanoid robot successfully navigating from a starting point through a multi-level 3D indoor environment to reach a specific target destination described in natural language.
Scene & Environment:
- The environment is a photorealistic, multi-story indoor space rendered in a "cutaway" or "dollhouse" style.
- At least one staircase connects the floors; it is the only way to change elevations.
- The destination may be located on any floor, so the robot might need to travel upstairs or downstairs mid-trajectory.
- The scene contains static obstacles such as walls, furniture (desks, chairs, couches), doorways, and stair railings.
- The environment and all objects within it (except the robot) are completely static.
- Preserve the existing scene layout, lighting, and furnishing exactly as provided; do not introduce, remove, or rearrange any elements.
- Destination Integrity: Keep the size, appearance, and placement of the described destination area exactly as it already exists in the provided scene.
- Floors and stair treads are the only navigable surfaces; there are no elevators, ramps, or floating platforms.
Agent & Goal:
- Agent (Start Point): A clearly mechanical humanoid robot (silver or white body panels, visible joints, illuminated visor/sensors) standing roughly 1.5-2 meters tall; it must look robotic, never human.
- Agent Orientation: Align the robot's "front" with the initial facing direction indicated by the provided start marker.
- Goal (Destination): render the destination faithfully without altering its layout or surroundings.
Rules of Movement & Visibility:
- The robot walks with a natural, bipedal gait. It does not slide, float, or teleport.
- The robot maintains a steady, consistent walking speed throughout the navigation.
- The robot obeys physical constraints: it cannot clip through or pass through solid objects.
- Stair Navigation: When moving between floors, the robot climbs or descends the staircase step-by-step, keeping its feet planted on individual treads.
- The robot must actively navigate around obstacles by finding a clear, plausible path across floors.
- The robot moves purposefully and efficiently toward the described destination and stops once it clearly reaches that location.
- Static Markers: The provided start marker and destination remain fixed; they do not move, fade, or disappear.
- Wall Fading: If architectural elements block the camera's view, they may fade or become transparent so the robot stays visible at all times.
Camera:
- Perspective: Show the motion from a single, static, third-person isometric view (a "dollhouse" view) that includes all relevant floors.
- Camera Motion: The camera does not move, pan, zoom, or rotate.
- Scene Motion: The humanoid robot is the only moving object in the video; every other element remains static.
- Video Quality: The video feed is clear, well-lit, photorealistic, and free of glitches, sensor noise, or digital artifacts.
\end{promptlisting}
\end{minipage}
\end{center}

\paragraph{Image Generation Prompt.}\label{sec:prompt_embodied_3d_image_gen}
\begin{center}
\begin{minipage}{0.95\textwidth}
\begin{promptlisting}
We provide four prompt variants tailored to different navigation scenarios:
Variant 1: COLOR_FLOOR01 (Single-floor navigation to red target)
Create a single photorealistic still image (or edit the provided dollhouse frame) that captures the final state of a humanoid robot finishing its navigation inside the single-floor cutaway scene.
Scene & Environment:
- Use the supplied cutaway or isometric panorama exactly as rendered-this is a fixed top-down-style 3D view. Do not move, rotate, or zoom the camera.
- Preserve every architectural element, piece of furniture, lighting cue, and the red goal marker exactly as provided. Because this is a color hard level, the red region's hue (#ff0000), texture, outline, and placement are the definition of the destination and must remain untouched.
- Only the robot and the trajectory overlay may change; all other details remain static.
Agent & Goal Status:
- Agent: Identify the humanoid robot visible in the input image, remove it cleanly from its starting pose, and place that same robot asset at its destination pose.
- Goal: A bright red (#ff0000) region already painted on the floor. Do not recolor, resize, reshape, or move this area; simply depict the robot standing fully inside or touching its edge to prove the destination is reached.
- Navigation Evidence: Draw a bright green (#00ff00) trajectory line that traces the plausible path from the original start position to the red goal while respecting walls and furniture; this line is the permanent record of how the robot navigated, so it must remain clearly visible from start to finish.
- After relocating the robot, restore the original start area so it shows only the untouched floor/marker with no duplicated robot silhouettes.
Image Requirements:
- Show a single finished moment - no motion blur, no multiple exposures, no animated cues.
- Maintain the fixed over-the-shoulder/isometric framing so viewers can read both the robot and the red goal simultaneously.
- Ensure lighting, shadows, and reflections on the robot align with the untouched environment so the edit feels seamless.
Variant 2: COLOR_FLOOR02PLUS (Multi-floor navigation to red target)
Create a single photorealistic still image (or edit the provided multi-floor dollhouse frame) that captures the final state of a humanoid robot finishing its navigation across stacked floors.
Scene & Environment:
- Work directly on the provided multi-level cutaway render. Keep the panels, stair locations, lighting, and red goal exactly as shown. The camera remains a locked, static top-down/isometric view.
- No walls, staircases, furnishings, or the red goal itself may be added, removed, recolored, or repositioned. In this color hard level, the existing red destination is the canonical target and must stay exactly as provided. Only the robot and trajectory overlay can change.
Agent & Goal Status:
- Agent: Locate the humanoid robot in the source image, remove it from the starting pose, and reinsert it at the final destination pose on the correct floor.
- Goal: The existing bright red goal patch. Never recolor, resize, or relocate this marker-only place the robot fully inside it (or touching its boundary).
- Navigation Evidence: Draw a continuous bright green trajectory that follows the robot's entire route, including the stair climb/descent. When the path crosses floors, bridge the segments at the staircase so viewers can follow the transition. Keep the full path visible as the definitive record of the navigation.
- Clean the previous start location so it shows only the untouched floor/marker with no lingering robot artifacts.
Image Requirements:
- Present a single static frame with no sequential panels or animation hints.
- Keep the fixed camera framing wide enough to show every relevant floor and the final pose simultaneously.
- Match lighting and shading on the relocated robot with the environment for a seamless composite.
Variant 3: OBJECT_FLOOR01 (Single-floor navigation to described location)
Create a single photorealistic still image (or edit the provided dollhouse frame) that captures the final state of a humanoid robot completing its navigation toward the location described as: **"<LOCATION_DESCRIPTION>"** inside a single-floor cutaway scene.
Scene & Environment:
- Use the provided isometric frame as-is. Do not reframe, relight, or modify the architecture, furniture, or described location.
- Only adjust the robot placement and overlay graphics needed to illustrate its trajectory.
Agent & Goal Status:
- Agent: Identify the humanoid robot in the input image, remove it from the original starting pose, and place the same asset at the described destination so it clearly interacts with **"<LOCATION_DESCRIPTION>"**.
- Goal: Depict the exact object/area from the description without adding artificial highlights; rely on accurate positioning to show success.
- Navigation Evidence: Draw a bright green (#00ff00) trajectory from the start marker to the described location, weaving around obstacles realistically.
- After relocation, retouch the initial position so only the untouched floor/marker remains, with no duplicate robot body.
Image Requirements:
- Keep the static third-person/isometric viewpoint fixed so the spatial relationship between the robot and the described target is clear.
- Ensure the robot looks settled (no blur) and that lighting/shadows match the untouched environment.
- The still should feel like the last frame of a navigation sequence, showing completion without motion cues.
Variant 4: OBJECT_FLOOR02PLUS (Multi-floor navigation to described location)
Create a single photorealistic still image (or edit the provided multi-floor dollhouse frame) that captures the final state of a humanoid robot completing its navigation toward: **"<LOCATION_DESCRIPTION>"** across stacked floors.
Scene & Environment:
- Operate directly on the supplied multi-level cutaway render. Preserve the panel arrangement, stair geometry, lighting, and the described destination exactly as they appear. The camera is fixed and must not change.
- Only the robot placement and path overlay are edited; all other scene elements remain untouched.
Agent & Goal Status:
- Agent: Detect the humanoid robot in the frame, remove it from the initial pose, and place the same asset at the described destination on the appropriate floor.
- Goal: Show the robot interacting naturally with the destination - standing beside, touching, or centered on the described area-without inventing new highlights.
- Navigation Evidence: Draw a bright green (#00ff00) trajectory that spans the entire route, including stair transitions, so viewers understand how the robot arrived.
- After moving the robot, restore the original start area so it blends seamlessly into the untouched environment.
Image Requirements:
- Retain the static dollhouse viewpoint that shows all necessary floors simultaneously.
- Depict a single, clean final frame - no motion blur, duplicates, or animation artifacts.
- Ensure the relocated robot's lighting and shadows match the surrounding scene for photorealistic integration.
\end{promptlisting}
\end{minipage}
\end{center}

\paragraph{Video Evaluation Prompt.}\label{sec:prompt_embodied_3d_video_eval}
\begin{center}
\begin{minipage}{0.95\textwidth}
\begin{promptlisting}
You are an expert evaluator for 3D real-world, third-person-view navigation videos. Judge whether the agent depicted in the generated video satisfies the navigation goal while preserving physical realism and instruction fidelity.

INPUTS YOU RECEIVE
1. INITIAL_IMAGE – a single RGB frame that shows the agent’s exact starting pose and surrounding layout.
2. LOCATION_DESCRIPTION(OPTIONAL) – a textual destination description provided only for hard “object” levels; otherwise this field may be empty or “NONE”.
3. NAVIGATION_VIDEO – a video generated by a model such as VEO3 or Sora2 that shows the entire navigation attempt.

GENERAL DIRECTIONS
- Treat the initial image as the authoritative starting state. Verify that the video begins consistently with this frame (agent pose, camera angle, nearby objects).
- Use the location description to pin down the correct destination semantics (object identity, relative placement, contextual cues). When no description is given, infer the intended goal from landmarks visible in the initial image plus the agent’s behavior.
- Watch the whole video carefully. If there is any ambiguity about collisions, teleports, or scene edits, assume the stricter (failing) interpretation and set the relevant metric to 0.
- Each metric is binary (0 or 1). Record 0 whenever evidence is missing, unclear, or contradicts the pass condition.
- The agent must obey physical constraints: it should walk through traversable space, cannot pass through solid objects, and must maintain temporal continuity.

METRICS (REFERENCE THE CRITERIA FILE)

1. SUCCESS_SCORE_3D
   - 1 if the agent reaches the described/marked destination and comes to rest inside it by the end of the video.
   - 0 if it never reaches, overshoots, keeps moving after arrival, or the destination cannot be confirmed.

2. ORACLE_SUCCESS_SCORE_3D
   - 1 if, at any point, the agent passes through or pauses within the correct goal region even if it fails to stop there permanently.
   - 0 if the agent never enters the destination vicinity.

3. OBJECT_SEMANTIC_SCORE
   - 1 if the agent never collides with or phases through solid objects such as furniture, walls, doors, or pillars.
   - 0 if any overlap, clipping, or impossible interaction occurs.

4. AGENT_CONSISTENCY_SCORE
   - 1 if the agent’s appearance, position, and orientation evolve smoothly without teleportation, scale jumps, or sudden pose resets.
   - 0 if any temporal discontinuity or impossible acceleration happens.

5. SPATIAL_ALIGNMENT_SCORE
   - 1 if heading, body orientation, and elevation changes remain physically coherent (turn-then-move, climb only when stairs/ramps exist, no floating between floors).
   - 0 if the agent moves in a direction inconsistent with its facing direction, drifts sideways without turning, or violates elevation logic.

6. DESTINATION_INTEGRITY_SCORE
   - 1 if the destination in the video matches the initial specification (visual location in the initial image and/or the textual location description) AND the agent finishes inside that unchanged goal.
   - 0 if the destination differs from the initial reference in any obvious way (moved, resized, recolored, swapped object, contradictory text match) or if the agent stops outside the intact destination.

7. SCENE_CHANGE_SCORE
   - 1 if the environment remains static aside from expected parallax (no objects/structures/lighting popping in or out).
   - 0 if any scene element is added, removed, or morphs during the video.

EVALUATION STEPS
1. Compare the initial image with the video’s opening frames to confirm continuity.
2. Identify the goal location using the description (if any) and visual cues.
3. Observe the entire trajectory for success proximity, collisions, teleportation, and spatial alignment violations.
4. Inspect the goal region for tampering or relocation by comparing the final destination to BOTH the initial image and the location description. Any mismatch sets DESTINATION_INTEGRITY_SCORE to 0, even if the agent stops there.
5. Note any scene-wide changes between frames.
6. Assign each metric a binary score based strictly on the definitions above.

OUTPUT FORMAT
Return ONLY a JSON object with two top-level sections:
1. `"SCORES"` – matches the exact metric format in task03_evaluation_output_format.txt (string values "0" or "1").
2. `"REASONING"` – a dictionary mirroring the metric keys; each value is a short sentence explaining why the corresponding score is 0 or 1 (cite concrete visual evidence).

Example schema:
{
  "SCORES": {
    "SUCCESS_SCORE_3D": "<0 or 1>",
    "ORACLE_SUCCESS_SCORE_3D": "<0 or 1>",
    "OBJECT_SEMANTIC_SCORE": "<0 or 1>",
    "AGENT_CONSISTENCY_SCORE": "<0 or 1>",
    "SPATIAL_ALIGNMENT_SCORE": "<0 or 1>",
    "DESTINATION_INTEGRITY_SCORE": "<0 or 1>",
    "SCENE_CHANGE_SCORE": "<0 or 1>"
  },
  "REASONING": {
    "SUCCESS_SCORE_3D": "<brief justification>",
    "ORACLE_SUCCESS_SCORE_3D": "<brief justification>",
    "OBJECT_SEMANTIC_SCORE": "<brief justification>",
    "AGENT_CONSISTENCY_SCORE": "<brief justification>",
    "SPATIAL_ALIGNMENT_SCORE": "<brief justification>",
    "DESTINATION_INTEGRITY_SCORE": "<brief justification>",
    "SCENE_CHANGE_SCORE": "<brief justification>"
  }
}
Do not include any other text outside this JSON object.
\end{promptlisting}
\end{minipage}
\end{center}

\subsection{Simultaneous Localization and Generation (SLAG)}

\paragraph{Video Generation Prompt.}\label{sec:prompt_embodied_slag_video_gen}
\begin{center}
\begin{minipage}{0.95\textwidth}
\begin{promptlisting}
Create a split-screen video for the task "Simultaneously Localization and Generation." The left panel must show a humanoid robot navigating a photorealistic 3D indoor scene, while the right panel simultaneously shows a generated 2D top-down map visualizing the exact trajectory in real time.
Panels & Layout:
- The frame is bisected vertically: LEFT = 3D dollhouse view, RIGHT = generated 2D map.
- Both panels remain visible, aligned, and synchronized from the first frame to the last; no fades, picture-in-picture, or camera cuts.
- Time is locked: every robot motion in the left panel updates the right-panel map at the same moment.
Left Panel - 3D Scene:
- Environment: a realistic indoor space (e.g., apartment, office) rendered as a fixed, cutaway dollhouse view with walls, furniture, and doors that never move.
- Agent: a clearly mechanical humanoid robot (silver/white panels, visible joints, glowing sensors) ~1.5-2 m tall.
- Start Marker: a bright blue (#0000ff) triangular decal on the floor that indicates the starting pose; the robot initially stands perfectly centered on the triangle with its "face" pointing toward the triangle's tip.
- Goal Region: a bright red (#ff0000) target area painted on the floor; it remains visible for the entire video.
- Constrain the robot to walk naturally, obeying physics (no clipping, sliding, teleporting) while following a purposeful path to the red goal.
- Keep the camera static, isometric, and wide enough to include the entire navigable layout. Fade obstructing walls only if they block the robot from view.
Right Panel - Generated 2D Map:
- Depict a clean, top-down schematic of the same environment: navigable space in white, obstacles/walls in dark gray or black, start triangle in blue, goal region in red.
- The map is generated/progressive: it begins with the static layout plus both markers, then draws a bright green (#00ff00) trajectory line that grows as the robot advances.
- Represent the robot as a top-down icon (matching the humanoid silhouette or a triangular arrow) whose orientation always points along the direction of travel and stays aligned with the 3D motion.
- Only the robot icon and the green trajectory move/change; all other map elements stay fixed.
Rules of Movement & Mapping:
- The robot maintains a steady walking speed, rotates its torso to face the current heading, and never moonwalks or strafes.
- The green line is continuous, accurately matching the robot's floor path without gaps, jumps, or intersections through walls.
- The task ends when the robot stands completely inside the red goal region; both panels freeze on that final pose for a brief beat with the full trajectory visible.
Camera & Rendering:
- No motion blur, glitching, or exposure shifts. Lighting is even and realistic.
- Aside from the robot, the left scene is entirely static. Aside from the robot icon and green path, the right map is entirely static.
- Ensure the two panels remain perfectly synchronized and visually consistent (wall layout, start/goal locations, total path length).
\end{promptlisting}
\end{minipage}
\end{center}

\paragraph{Image Generation Prompt.}\label{sec:prompt_embodied_slag_image_gen}
\begin{center}
\begin{minipage}{0.95\textwidth}
\begin{promptlisting}
We provide four prompt variants tailored to different navigation scenarios:
Variant 1: COLOR_FLOOR01 (Single-floor navigation to red target)
Create a dual-panel photorealistic still image (or edit the provided split frame) that captures the final moment after the humanoid robot completes its navigation inside the single-floor environment.
Panels & Layout:
- Keep the vertical split exactly as provided: LEFT = 3D dollhouse view, RIGHT = generated 2D map.
- Both panels must stay perfectly aligned and synchronized. Do not crop, reposition, or recolor either half, and never introduce fades or picture-in-picture effects.
Left Panel - 3D Scene:
- Use the supplied cutaway render without moving the static isometric camera. Identify the humanoid robot already present, remove it cleanly from the initial blue (#0000ff) triangle, and place the same asset at the final pose standing fully inside the bright red (#ff0000) goal patch. The red region defines the destination in color hard levels, so never recolor, resize, or relocate it.
- Overlay a bright green (#00ff00) trajectory that traces the exact path from the blue triangle to the red goal, respecting walls and furniture. This path must remain clearly visible as the permanent navigation record.
- After relocating the robot, restore the starting area so only the untouched floor/triangle marker remains-no duplicate robot silhouettes or shadows.
Right Panel - Generated 2D Map:
- Preserve the existing top-down schematic (white walkable space, dark obstacles) and keep the static camera framing untouched.
- Move the robot icon (humanoid outline or arrow) from its starting position to the final cell that corresponds to the red goal shown on the left. Do not invent additional destination markers; if the map lacks a red patch, simply terminate the path at the coordinate aligned with the left-panel goal.
- Draw the complete bright green (#00ff00) trajectory that mirrors the left-panel route, including turns. The start triangle remains blue but now stands empty; only the robot icon and path should change.
Image Requirements:
- Depict a single final frame with no motion blur or sequential panels.
- Lighting, materials, and annotations must stay consistent with the source image.
- Ensure both panels visually agree on floor layout, start/goal placement, and total path length.
Variant 2: COLOR_FLOOR02PLUS (Multi-floor navigation to red target)
Create a dual-panel photorealistic still image (or edit the provided split frame) that captures the final moment after the humanoid robot completes its navigation across stacked floors.
Panels & Layout:
- Preserve the vertical split exactly as provided. The left panel shows the multi-floor dollhouse, and the right panel shows the synchronized multi-floor 2D map; keep both fully visible and aligned.
Left Panel - 3D Scene:
- Keep the static isometric camera and multi-floor cutaway exactly as delivered. Identify the humanoid robot, remove it from the initial blue (#0000ff) triangle, and reinsert it at the final pose on the correct floor, standing fully inside the bright red (#ff0000) goal patch. Never alter the red destination marker-it is the canonical target for color hard levels.
- Overlay a continuous bright green (#00ff00) trajectory from the start marker through all traversed floors to the goal. When the route uses stairs, run the path along the staircase so the elevation change is obvious. Leave the full trajectory visible end-to-end.
- Clean the original start location so the blue triangle is empty and the floor looks untouched aside from the persistent marker.
Right Panel - Generated 2D Map:
- Maintain the existing multi-floor schematic (stacked top-down slices). Do not reposition floors or modify the camera.
- Move the robot icon to the final cell that corresponds to the left-panel goal. If the map does not contain a separate red marker, end the green path at the coordinates that align with the left-panel destination rather than inventing a new decal.
- Draw the entire bright green (#00ff00) trajectory across every slice, bridging between floors at the staircase connections so viewers can trace the vertical transitions. Only the robot icon and path should update; all other map graphics remain static.
Image Requirements:
- Show a single completed moment with no animation cues.
- Ensure the geometry, stair locations, and total travel distance match between panels.
- Lighting, shadows, and rendering style must remain faithful to the original inputs.
Variant 3: OBJECT_FLOOR01 (Single-floor navigation to described location)
Create a dual-panel photorealistic still image (or edit the provided split frame) that captures the final moment after the humanoid robot reaches the location described as: **"<LOCATION_DESCRIPTION>"** inside a single-floor environment.
Panels & Layout:
- Retain the original left/right layout and keep both panels synchronized; do not reposition the split or adjust camera settings.
Left Panel - 3D Scene:
- Use the supplied dollhouse render without changing the static camera. Identify the humanoid robot, remove it from the starting pose on the blue (#0000ff) triangle, and place the same asset beside or directly on the destination described by **"<LOCATION_DESCRIPTION>"**. Do not add artificial highlights; rely on accurate placement and natural contact.
- Draw a bright green (#00ff00) trajectory from the start marker to the described location, weaving naturally around furniture. Keep the full path visible as the navigation record.
- After relocation, ensure the initial blue triangle is unoccupied and the floor underneath looks untouched.
Right Panel - Generated 2D Map:
- Keep the static top-down schematic unchanged aside from updated robot/path overlays. The map should reflect the same destination as the left panel; label the described location subtly (e.g., thin outline or text) only if the source already includes it-do not fabricate new symbols.
- Move the robot icon to the cell corresponding to **"<LOCATION_DESCRIPTION>"**, and draw the matching bright green (#00ff00) trajectory from the start triangle to that cell. The path must mirror the 3D route exactly.
- Clean up the starting position so only the blue triangle remains while the robot icon appears solely at the destination.
Image Requirements:
- Present one final frame with no motion blur. Both panels must agree on geometry, destination placement, and total path length.
- Maintain all original lighting, materials, and map styling.
Variant 4: OBJECT_FLOOR02PLUS (Multi-floor navigation to described location)
Create a dual-panel photorealistic still image (or edit the provided split frame) that captures the final moment after the humanoid robot reaches the destination described as: **"<LOCATION_DESCRIPTION>"** across stacked floors.
Panels & Layout:
- Keep the vertical split and panel alignment exactly as provided so the multi-floor dollhouse and the multi-slice map stay synchronized.
Left Panel - 3D Scene:
- Use the provided multi-level cutaway without altering the static camera. Identify the humanoid robot, remove it from the start marker on the lower floor, and place the same asset at **"<LOCATION_DESCRIPTION>"** on the correct floor, showing natural contact and orientation.
- Overlay a bright green (#00ff00) trajectory from the blue triangle through every stair segment to the described location. Leave the entire route visible to document the navigation.
- Once the robot is relocated, the original start marker must be empty with only the static triangle remaining.
Right Panel - Generated 2D Map:
- Preserve the stacked floor slices exactly. Move the robot icon to the cell aligned with **"<LOCATION_DESCRIPTION>"** and, if the source map already marks that location, keep the notation consistent; otherwise, end the path at the coordinate without inventing new symbols.
- Draw the matching bright green (#00ff00) trajectory across all slices, connecting floors at staircase locations so the vertical movement stays legible. Only the robot icon and trajectory should change.
- Make sure the start triangle is left unoccupied after relocation.
Image Requirements:
- Deliver a single, crisp final frame with no animation cues.
- The geometry, stair usage, and total travel distance must line up between the panels.
- Preserve original lighting, materials, and map palette to ensure the edit remains seamless.
\end{promptlisting}
\end{minipage}
\end{center}

\paragraph{Video Evaluation Prompt.}\label{sec:prompt_embodied_slag_video_eval}
\begin{center}
\begin{minipage}{0.95\textwidth}
\begin{promptlisting}
You are an expert evaluator for Simultaneous Localization and Generation. Every sample provides:
1. TASK_DESCRIPTION – textual reminder of the navigation objective, start, and goal.
2. NAVIGATION_VIDEO – a synchronized split-screen clip:
   • LEFT panel: a fixed “dollhouse” 3D render showing the humanoid robot walking through the actual environment, with blue start and red goal highlights.
   • RIGHT panel: a progressively drawn 2D map using the same blue start marker, red goal footprint, robot icon, and bright green trajectory.
3. LOCATION_DESCRIPTION(OPTIONAL) – a textual destination description provided only for hard “object” levels; otherwise this field may be empty or “NONE”.
Your job is to verify that both panels depict the same physically plausible run, that the robot reaches the intended destination, and that mapping/localization stay consistent.

GENERAL DIRECTIONS
- Treat the two panels as perfectly synchronized observations. Any mismatch in pose, timing, or goal location counts against the relevant metric.
- All metrics are binary (1 = pass, 0 = fail). When evidence is missing, ambiguous, or contradictory, default to 0.
- Use the formal definitions summarized below from `task04_evaluation_criteria.txt`, and report results strictly in the schema defined by `task04_evaluation_output_format.txt`. Do not invent extra commentary or alternative scores.

METRICS (apply these literal criteria)
1. SUCCESS_SCORE_2D – 1 only if the right-panel map shows the green trajectory ending with the robot icon fully inside the red goal footprint when the video stops; otherwise 0.
2. ORACLE_SUCCESS_SCORE_2D – 1 if the 2D trajectory ever intersects or brushes the red goal, even if the final state is elsewhere; otherwise 0.
3. TRAJECTORY_ALIGNMENT_SCORE – 1 when the path drawn in the 2D map mirrors the physical path in 3D (same turns, segment lengths, obstacle avoidance, no impossible gaps/teleports); otherwise 0.
4. SUCCESS_SCORE_3D – 1 if the humanoid in the 3D panel halts inside the red goal region at the end; otherwise 0.
5. ORACLE_SUCCESS_SCORE_3D – 1 if the 3D robot ever reaches/touches the goal area at any point, regardless of the final stop; otherwise 0.
6. OBJECT_SEMANTIC_SCORE – 1 when the agent never collides with or phases through solid geometry/furniture and the 2D path never routes through obstacles; otherwise 0.
7. AGENT_CONSISTENCY_SCORE – 1 if motion stays temporally continuous with no teleporting, pose pops, or scale jumps in either panel; otherwise 0.
8. SPATIAL_ALIGNMENT_SCORE – 1 if heading, stride direction, and elevation changes are coherent (no moonwalking, strafing, or floating) and the 2D icon orientation matches the 3D heading; otherwise 0.
9. DESTINATION_INTEGRITY_SCORE – 1 when the start/goal markers remain fixed, unedited, and the robot finishes within the original red goal in both panels; otherwise 0.
10. SCENE_CHANGE_SCORE – 1 if the environment (walls, furniture, lighting) and the static components of the 2D map stay unchanged for the full clip; otherwise 0.

EVALUATION STEPS
1. Read the TASK_DESCRIPTION to understand the intended destination and layout constraints.
2. Watch the split-screen video end-to-end, monitoring synchronization between panels.
3. Track the robot’s motion for collisions, teleportation, or heading inconsistencies while confirming the 2D path mirrors every 3D turn.
4. Inspect the start/goal markers and surrounding environment for any edits or relocations.
5. Assign each metric strictly per the definitions above, defaulting to 0 when uncertain.

OUTPUT FORMAT
Return ONLY a JSON object with:
- "SCORES": matches the exact key/value schema in `task04_evaluation_output_format.txt`, using strings "0" or "1".
- "REASONING": repeats every key with a brief justification citing observations from the video.
Do not include extra commentary outside this JSON object.
\end{promptlisting}
\end{minipage}
\end{center}

\subsection{Physical Commonsense}

\paragraph{Video Generation Prompt.}
\begin{center}
\begin{minipage}{0.95\textwidth}
\begin{promptlisting}
We provide the model with a detailed text prompt describing a specific physical scenario. The prompts are designed to test physical understanding through concrete scenarios that have physically correct (or incorrect) outcomes. Examples span both Physical Concepts and Sports Scenarios:
Physical Concepts (Solid-Solid): "A blender spins, mixing squeezed juice within it."
Physical Concepts (Solid-Fluid): "A brave diver splashes into a pool from a great height."
Physical Concepts (Fluid-Fluid): "Honey diffusing into warm milk."
Sports Scenarios (Ballet): "A ballet dancer performs a graceful pirouette, maintaining perfect balance and rotational momentum throughout the spin."
Sports Scenarios (Skiing): "A skier navigates down a steep mogul field, their body absorbing the bumps while maintaining forward momentum and control."
Sports Scenarios (Diving): "An Olympic diver executes a pike position dive from the 10-meter platform, rotating smoothly before entering the water with minimal splash."
Sports Scenarios (Swimming): "A swimmer performs a butterfly stroke, coordinating arm movements with dolphin kicks to propel through the water efficiently."
\end{promptlisting}
\end{minipage}
\end{center}
